# Supplementary material for: Stereo-Knowledge Distillation from dpMV to Dual Pixels for Light Field Video Reconstruction
Source: arXiv:2405.11823 source file (2024-05-20)
Supplement: Supplementary file 1 [file supplementary.tex]

% Manage supplementary from this file

\section*{Supplementary Structure}
\label{sec:supp}

\begin{itemize}
    \item \textbf{Contributions and Taxonomy} (\cref{sec:contributions}): Here, we provide a review of our contributions, outlining the taxonomy and advantages of our method.
    
    \item \textbf{Reproducibility} (\cref{sec:reproducability}): Here, we provide more details about this work hosted at~\href{https://github.com/ANonyMouxe}{https://github.com/ANonyMouxe} and provide a correction \& addendum to the main text.
    
    \item \textbf{Motivation.} (\cref{sec:dp_explained_dof}): We begin by elucidating the motivation behind addressing the challenge of dual pixels within the depth-of-field, utilizing our dark knowledge distillation hypothesis.
    
    \item \textbf{Extended Related Work} (\cref{sec:extended_related}): We delve into an expanded review of related work, building upon the discussion in the main paper.
    
    \item \textbf{Dark Knowledge Distillation for DP-Disparity Estimation} (\cref{sec:dark}): This section presents a conventional paper-style breakdown. We discuss dark knowledge distillation, methodology, implementation details, and experiments, including comparisons, ablations, and a limitation (\cref{fig:dark_dp_limitation}). We present the dpMV \textit{benchmark} in Table~\ref{tab:benchmark_dpmv}.
    
    \item \textbf{Light Field Video Reconstruction} (\cref{sec:lfvr_supplement}): Here, we provide an in-depth exploration of our light field video reconstruction method, covering teacher-selection procedure, dual pixel simulation, theoretical underpinnings, additional results, experiments, and extensive applications of our light field reconstructions (\cref{fig:xr_applications}, \cref{fig:refocus} and \cref{fig:nvs_all}).
    We conclude this section with a comprehensive discussion on the limitations of our proposed method and suggest potential solutions.

    \item \textbf{dpMV Dataset Samples} (\cref{sec:dataset}):
    This section displays all of the indoor-outdoor classes with a separate display of the non-Lambertian, visible light sources and transmissive or highly reflective surfaces. 
    One to two-word captions that accompany each video enable also enable dual-pixel or multi-view image/video classification, captioning and other multi-modal learning-based tasks.
    
\end{itemize}

\section{Contributions}
\label{sec:contributions}
Overall, we contribute a central distillation idea for the computational imaging field, 4+1 \textit{dp}-models that perform camera depth-of-field aware disparity estimation and light field video reconstruction, using the distillation hypothesis, and a first-of-its-kind large dual pixel multi-view videos (\textit{dp}MV) dataset.

\subsection{Novelty.}
\begin{enumerate}
    \item \textit{Central Hypothesis of the paper.} Dark Knowledge distillation, implicit or explicit, from synthetically pre-trained stereo methods to dual pixel networks.
    
    \item \textit{dpMV dataset} to push methods using our hypothesis and other dual pixel and multi-view tasks including classification, captioning and multi-modal learning as the dataset comes with classes and 1-to-2 word captions as well.
    
    \item Validation of the hypothesis on disparity estimation task while \textit{benchmarking} dpMV. Here, 4 dark-dp-disparity networks are contributed.
    
    \item An application of the implicit version of the hypothesis is demonstrated for \textit{single dp-view light field video reconstruction}, for the first time.

    \item The first use case of vision transformers for light field reconstruction.

    \item LF reconstruction achieves the lowest inference time while maintaining the highest video temporal consistency.
\end{enumerate}

% b) The \textbf{58,295 frames' dual-pixel video dataset captured in dynamic environments. The dataset also has additional rectified \& synchronized stereoscopic views}. 
% The multi-view dataset enables conventional vision tasks in addition to providing researchers the opportunity to solve the same tasks with the ubiquitous dual-pixels (found in most smartphones nowadays) using \textbf{the cross-modal pretext (additional views), thus encouraging self-supervised research}.  
% \textbf{b) We contribute the first method for LF reconstruction using dual pixels}. 

% c) We also show \textbf{the first use case of vision transformers (ViT) for LF reconstruction}. 
% The zero-shot cross-data, angular \& spatial characteristics, while being competitive with the prior refinement-based supervised methods and state-of-the-art without supervision, demonstrate the superiority of our novel architectural choice, design, and training setup. 
% These choices were based on the \textbf{key insight} that the dual pixels could provide implicit disparity cues essential for LF reconstruction while also finely guiding the network along tricky edges (See Figure 6).  

% d) Our method also has the \textbf{lowest inference time and requires no extra inputs unlike most LF methods}.

\subsection{Significant Differences \& Advantages over Monocular and Stereo Light Field State-of-the-Art Methods}
While our work shares some similarities with Mono~\cite{eccv_22_monoLFVR} and SelFVi~\cite{Selfvi}, significant differences distinguish our approach, leading to substantial improvements over these methods.
To name a few, generalization or zero-shot properties, speed, parameter efficiency, no extra hardware calibration, no post-processing costs, no external network dependencies, and no need for ground truth light fields for refinement are some crucial gains arising from our method.
On a deeper level, our approach solves the hardest task of truly understanding the 3D scene while being hardware-practical:

\textbf{Difficulty of task.}
SeLFVi computes disparity from its stereo input explicitly unlike our implicit methods for computing the disparity plane centers. 
While we predict disparity planes using just the dual pixel input, Mono relies on explicit disparity estimates as input from an external pretrained DPT-384-Large~\cite{Ranftl2020}).
This provides Mono's network explicit 3D context and never is encouraged to capture the critical question "What does the 3D world look like" (Input Ablation Table and Input Ablation Breakdown section in the main text).
Our method is encouraged to do so through the distillation losses.

\textbf{Difficulty of Geometric Consistency.}
SeLFVi has to reconstruct one less sub-aperture view while also getting a better geometric consistency loss as the left view becomes the left-most SAI while the right view becomes the center SAI of the predicted light field for their method. 
Our method only has the central view but not the explicit disparity input (like Mono). 
Mono learns a simple pixel re-arrangement relation using the RGB + disparity input used during inference. 
For ours, a true 3D scene understanding is essential for correct SAI reconstruction (warping and hole-filling from single view) during inference.

\textbf{Ease of and load on hardware.}
Our exclusive use of RGP+DP channels eliminates smartphone deployment impracticalities for stereo cameras. 
Our ViT-based model has state-of-the-art inference times (Table 4) and is extremely parameter efficient with generalization capabilities across different types of datasets (or scenes) and user-defined settings like LF spatial-angular resolution, and baseline. 
Mono is resource-consuming, and impractical for user applications, especially due to the external massive depth-network \textit{required} during inference. 
Also, Mono does not generalize across datasets without the refinement module (fully supervised on GT LFs).

\textbf{Appropriateness of Vision Transformers for (dense) light field reconstruction} 
The synergy of dual pixels and ViT enables us to streamline reconstruction without explicit disocclusion handling, providing an efficient 3D scene understanding. 
The dual pixels play a guiding role in the reconstruction along edges (Fig. 6) and also provide imperative disparity cues without which the model never converges due to limited representational power and compute resources (Input side ablation Table in main paper). 

\subsection{Note on Cross-Modal Self-Supervision Taxonomy}
According to Jaiswal~\etal~\cite{rebuttal_01}, our method falls under cross-modal-pretext self-supervised learning (SSL) tasks, defined therein as follows: "Pretext tasks are self-supervised tasks that act as an important strategy to learn representations of the data using pseudo labels. These pseudo labels are generated automatically based on the attributes found in the data." 
Cross-modal is the additional view $I_A$ used to compute a stereo disparity estimate ($d_{st}$) or the pseudo-label computed from attributes ($I_A$) found in the dataset. 
Rani~\etal~\cite{rebuttal_02} uses the same operational definition by using a task-level classification: auxiliary pretext tasks and pseudo labels therein. 
Also, we never captured or had access to ground truth light fields to begin with so it rules out semi-supervised or weakly-supervised regimes that rely on partially labeled (GT) data to make sense of the unlabelled data during training. 
\section{Reproducibility}
\label{sec:reproducability}
The codebase for this paper is organized into three separate repositories (anonymous for now): 
Light Field Video Reconstruction, Dark tiny-dp-disparity networks and the Tuned-geometry-teacher in \href{https://github.com/ANonyMouxe/dp-LFVR}{dp-LFVR}, \href{https://github.com/ANonyMouxe/dark-dp-nets}{dark-dp-nets} and \href{https://github.com/ANonyMouxe/Dark-Knowledge-Tuned-Geometry-Teacher}{Dark-Knowledge-Tuned-Geometry-Teacher}.

\textbf{LFVR Implementation detail correction and addendum.} The light field reconstruction method uses a \textit{simulated} batch size of 16 using gradient accumulation instead of an actual batch size of 1. 
\textit{Addendum.} A fully PyTorch-Lightning codebase with DeepSpeed Zero-Offloading~\cite{ren2021zerooffload} for horizontal and extremely efficient sharding is under development and will be released upon publication.
\section{Motivation. Dual Pixels: A Boon and a Bane }
\label{sec:dp_explained_dof}

\textbf{Disparity Formulation in Dual Pixels.}
The disparity for a stereo pair with baseline $B$ at pixel $(x,y)$ in the left camera is given by $d^{st}_{x,y} = Bf/z$, where z is the depth at the pixel and $f$ is the focal length.
However, due to the introduction of the micro-lenslet array over the pixel sensor board and under the main lens, in addition to the tiny baseline of dual pixels, the equation for the disparity, similarly defined by Kim~\etal~\cite{spatio_bifocal} using the circle-of-confusion size ($b$), is given by: 
\begin{equation}
    d^{dp}_{x,y} = \alpha b = \alpha \frac{Af}{1 - f/z_f} (\frac{1}{z_f} - \frac{1}{z}) = p + \frac{q}{z}
    \label{eq:dp_disparity_equation}
\end{equation}
where, $A$ is the size of the main lens aperture, $z_f$ is the depth of the focus plane, $\alpha$ is a positive scale factor (\cref{fig:dp_dof_explainer}).
Note that this equation is affinely related to depth contrary to the stereo setup where they are directly inversely proportional.
We also solve for affine parameters for each dual-pixel disparity baseline and the inverse relation for monocular depth estimation to get affine-invariant metrics for disparity estimation in~\cref{tab:benchmark_dpmv}.

Nevertheless, when a camera operates in ultra-large depth-of-field or all-in-focus settings ($b \rightarrow 0$), dual pixel disparity is negligible ($d^{dp}_{x,y} \rightarrow 0$). 
This limitation necessitates capturing with \textit{defocus blur} to get disparity information~\cite{spatio_bifocal, refocus_wadwa_18}. 
This is not the case with stereo-camera setups to estimate disparity.
So, this necessitates the exploration of a solution that can utilize the dual pixel hardware while reaching stereo-accuracy in \textit{all} camera operating conditions. 

\begin{figure}[t]
    \centering
    \includegraphics[width=\columnwidth]{supp_imgs/dual_pixels/dual_pixel_explainer.png}
    \caption{\textbf{Dual Pixels have disparity \textit{only} in out-of depth-of-field of the camera or defocus deblur regions.} Image Courtesy: Kim~\etal~\cite{spatio_bifocal}}
    \label{fig:dp_dof_explainer}
\end{figure}

\textbf{Machine Learning for the Best of Both.}
The drawback of dual pixels is the need to capture with defocus blur. 
However, this might not always be possible with proprietary camera ISPs that stabilize and aim for all-in-focus shots.
Stereo camera setups need perfect synchronization and the hardware needed for integration in a small-scale device like a smartphone is plentiful, making it impractical even if it is more accurate.
Machine learning delivers the best of both worlds by distilling knowledge from stereo networks to dp-networks.
This helps dp-networks to understand the depth-of-field of the camera and utilize appropriate channels (RGB for within depth-of-field and dp for out-of depth-of-field). 
\section{Extended Related Work}
\label{sec:extended_related}
\subsection{Disparity Estimation}
We surveyed three input-type methods for disparity estimation: monocular, dual-pixel, and stereo input.
The stereo-input methods were surveyed to select optimal dark-teachers for our distillation hypothesis while the others serve the purpose of baselines or noteworthy ideas.
We omit multi-view stereo methods like COLMAP~\cite{colmap_COLMAP}.

\textit{Monocular Depth Estimation Methods.}
Since disparity and depth are inversely proportional and can be estimated to a relatively accurate degree, we use and find in literature, mostly depth-based networks including the likes of Dense Prediction Transformer by Ranftl~\etal~\cite{Ranftl2020}, MiDaS~\cite{midas}, AdaBins~\cite{AdaBinsBhat} and ZoeDepth~\cite{zoeDepth}, both by Bhat~\etal.
The recent massively yet weakly supervised method Depth-Anything~\cite{depth_anything} method is by far the highest fidelity. 
We use it as a baseline for comparison.

\textit{Dual Pixel Methods.}
With the ubiquity of dual-pixel sensor smartphones, originally for auto-focusing, interest has risen in extracting disparity arising from the defocus blur.
DDDNet~\cite{Pan_2021_CVPR_DDDNet_DP_Disp}, DPNet~\cite{GargDualPixelsICCV2019_DPNet}, and DPDNet~\cite{abuolaim2020defocus_michaelBrownECCV} explored neural-network-based approaches.
While, Xin~\etal~\cite{Xin_2021_ICCV_dual_pixel_cmu}, DPDD~\cite{punnappurath2020modeling}, Wadhwa~\etal~\cite{refocus_wadwa_18} and Kim~\etal~\cite{spatio_bifocal} are purely optimization-based approaches thus requiring no-training data or a neural network.
Kim~\etal recently outperformed most optimization-based methods.
We contribute 4 mobile performant dp-disparity estimation neural network solutions using our dark knowledge distillation hypothesis.

\textit{Stereo Methods}
Disparity estimation or stereo matching has been a long-standing problem in computer vision and relies on effective feature matching and triangulation. 
Many deep learning-based methods have emerged that rely on warping, feature matching, cost-volume regression etc. 
Some methods include: ACVNet~\cite{xu2022attention_ACVNet}, Graft-PSM~\cite{graft_psm_net}, IGEV~\cite{xu2023iterative_igev}, CFNet~\cite{CF_Net_disp}, PSMNet~\cite{psmNet}, GA-Net~\cite{GA_Net}, AANet~\cite{AANet}, RAFT-Stereo~\cite{raft_stereo} and CREStereo~\cite{creStereo}.
Even transformer-based methods like STTR~\cite{STTR} and Unimatch or GMStereo~\cite{xu2023unifying_unimatch} exist. 
Unimatch won the Argoverse Challenge (CVPR-Workshop 2022 Autonomous Driving Challenge) even though it was pretrained on a synthetic dataset~\cite{sceneflow_dataset} thus showing remarkable real-world domain adaptation. 
This transformer-based network was fitting and unconstrained, thus making it a \textit{highly suitable} candidate for our \textit{dark knowledge geometry teacher} in the light field reconstruction task.

\begin{figure*}[ht]
    \centering
    \includegraphics[width=0.9\textwidth]{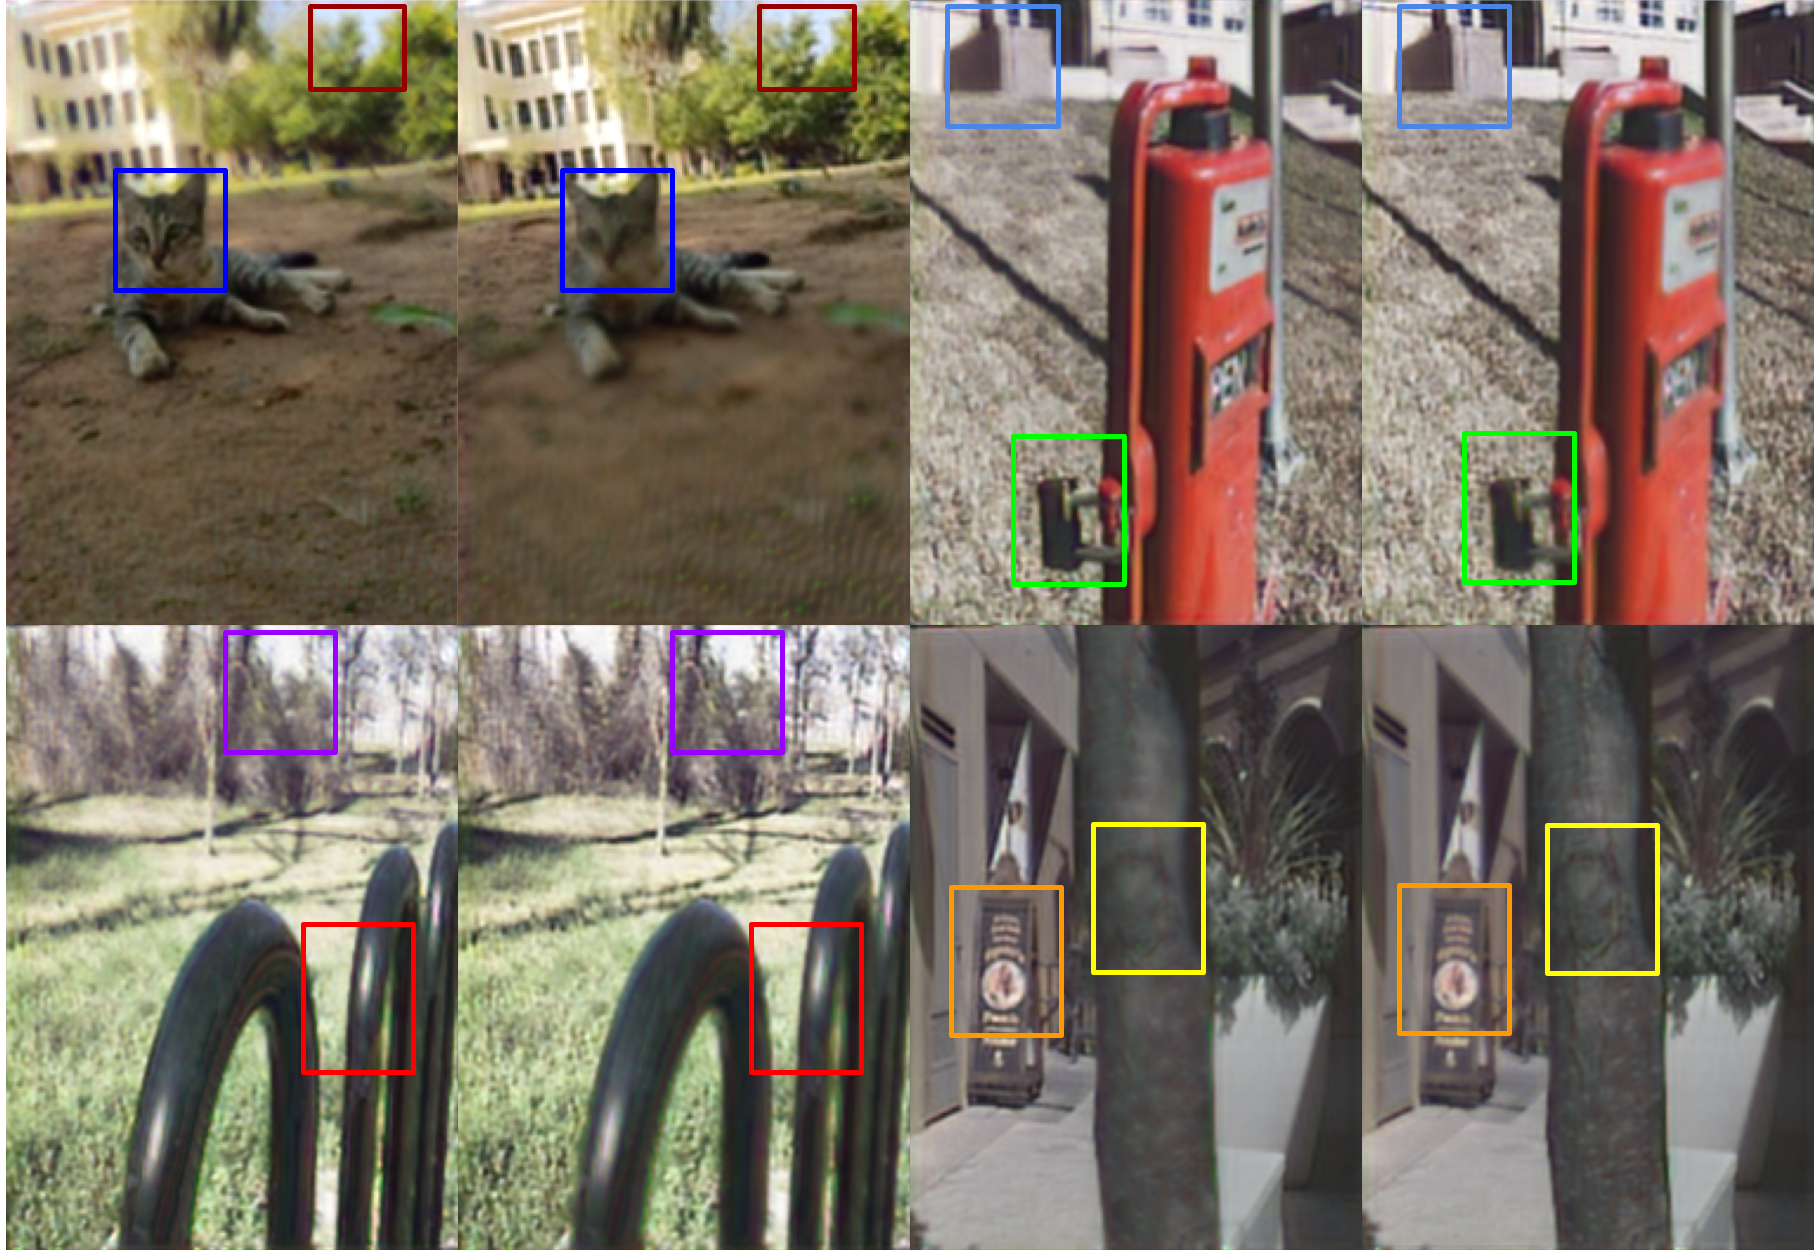}
    \caption{\textbf{Refocusing of our reconstructed light fields}. Note that the cat scene is from dpMV with real dual pixels while the others are from simulated dp-channels (GT LFdatasets)}
    \label{fig:refocus}
\end{figure*}

\subsection{Radiance Fields versus Light Fields}
\label{subsec:lf_vs_rf}
Even though Mildenhall \etal introduced the Local Light Field Fusion method \cite{LocalLF_fusion_2020} which eventually led them to an alternate, higher-fidelity seminal approach for novel view synthesis using radiance fields, colloquially known as NeRFs~\cite{mildenhall2020nerf, du2021nerflow, Dynamic_NeRF_Facial_Avatar, space_time_NeRF, dNeRF}, these approaches require integration along the rays to compute the intensity and opacity of a point in 3D space leading to a significant inference-time overhead. 
Additionally, a large set of overlapping inputs (upwards of 25) and cumbersome manual pre-processing using COLMAP for camera-pose estimation plagues them too. 
This is not practical for real scenarios where the user has a single shot at capturing a scene, for example, a flying bird.
Although, methods like pixelNeRF \cite{yu2021pixelnerf} and SinNeRF \cite{Xu_2022_SinNeRF} are singular view-based RF methods, they either work on simplistic objects or have prohibitive pre-training and inference times of up to 12 hours per scene. 
This significant time translates to all other downstream post-processing applications for every scene as NeRFs overfit/optimize MLPs to a scene. 
This makes RF-based methods totally infeasible for on-device applications whereas LF-based methods infer unseen scenes within mili-seconds. 
There have been significant efforts to eliminate this time drawback of RF methods and most speed-ups reduce the sampling points along a ray, but the issue of iterative sampling during ray-marching still persists. 
Recognizing this drawback, Wang \etal \cite{rf_2_lf} distilled an implicit 3D representation from a conventional NeRF model to a Neural LF model. 
Wang \etal observed a 30$\times$ speed-up with higher fidelity reconstructions but still needed intensive computations. 
InstantNGP~\cite{mueller2022instant_ngp},  MipNeRFs \cite{barron2021mipnerf} and the recent seminal 3D Gaussian Splatting method by Kerbl \etal \cite{kerbl3Dgaussians} present high-fidelity $120$+ fps renderings but still require an initial camera-pose estimation or 3D point cloud initialization. 
Per-scene optimization times of at least 20 minutes on sophisticated high-end graphics hardware are simply not possible for current smartphones, thus reiterating the practicality of learning explicit light fields as significantly faster and qualitatively better alternatives for non-deforming scenes~\cite{yu2023dylin}. 
To that end, we present the fastest Light Field Reconstruction method.

\subsection{Resurgence of Light Field Displays}
Light Fields have garnered interest mostly due to the availability of 3D-viewing hardware or 3D displays like Fovi3D, LumiPad and AR glasses from CREAL which are purely based on LF technology and enable interactive control (XR) as well.

\section{Dark Knowledge Distillation to dp-Disparity Networks}
\label{sec:dark}

% \begin{figure*}[h]
%     \centering
%     \includegraphics[width=0.9\textwidth]{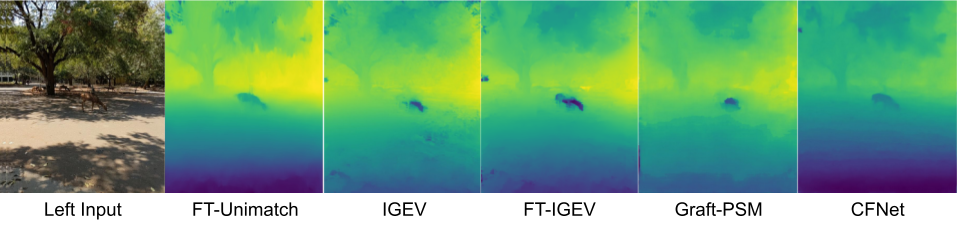}
%     \caption{\textbf{Dark Knowledge Stereo Disparity Teacher Selection.} $FT$ stands for hyper-parameter fine-tuned. 
%     Note that ACVNet~\cite{xu2022attention_ACVNet} and STTR~\cite{STTR} were also tried on the scenes of \textit{dp}MV but performed poorer than the shown methods.
%     The stereo teacher selected here is also used as the geometry teacher for our light field video reconstruction method (\cref{sec:lfvr_supplement})}
%     \label{fig:teacher_selection}
% \end{figure*}

\begin{table*}[ht]
    \caption{\textbf{Quantitative Comparison and \textit{dp}MV Benchmark} with Our Dark \textit{dp}-Disparity Estimators. 
    All Wall clock times ($W_{GPU}$ and $W_{CPU}$), per estimation, are in mili-seconds measured on a single NVIDIA RTX 3090.
    Parameters ($Params$) are in millions. 
    Even though MiDaS is significantly smaller and faster than DPT-Large-384, it is prone to a massive fidelity drop of close to $76\%$ compared to the same.}
    \centering
    \begin{tabular}{lccccccc}
    \toprule
    % Choose best metrics (left our rn: log-RMSE, Sq_Rel, \del < 1.25^2)
        Method & AI(1) & AI(2) & Params  & $W_{CPU}$ & $W_{GPU}$  \\
        \midrule \midrule
        Depth-Anything~\cite{depth_anything} & 0.212 & 0.261 & 335.3 & $>$20000 & 72.38 \\     
        DPT-Large~\cite{Ranftl2020} & 0.196 & 0.231 & 344.05 & 11770.71 & 17.63 \\  
        MiDaS~\cite{midas} & 0.237 & 0.304 & 21.32 & 427.31 & 13.82 \\     
        \midrule  
        DDDNet~\cite{Pan_2021_CVPR_DDDNet_DP_Disp} & 0.298 & 0.389  &  10.964  & 4223.05 & 73.34 \\    
        DPDD~\cite{punnappurath2020modeling} & 0.221 & 0.341 & - & $>$20000 & - \\  
        \midrule
        \textbf{Ours-Mv2} & 0.148 & 0.191 & \textbf{6.824} & 193.21 & 15.04 \\
        \textbf{Ours-Mv3-CPU}  & 0.182 & 0.215 & 6.916  & \textbf{173.96} & 17.71 &  \\ 
        \midrule
        \textbf{Ours-R34-{GPU}} & 0.129 & 0.169 &  26.08 & 538.26 & \textbf{11.20} \\
        \textbf{Ours-R50-Best} & \textbf{0.129} & \textbf{0.165}  & 48.98 & 1508.89 & 21.67 \\ 
    \bottomrule
    \end{tabular}
    \label{tab:benchmark_dpmv}
\end{table*}

\subsection{What is Dark Knowledge?}
Rich Caruana~\etal~\cite{kd_first_01} showed how to \textit{distill} knowledge from an ensemble of large models to a small or compressed model.
Subsequently, Geoffrey Hinton~\etal~\cite{kd_first_02} argued that transferring knowledge from a large general yet cumbersome model to a smaller network using \textit{temperature raised soft logits} (in classification task context) enables better smaller model performance. 
This temperature-scaled output from the larger model or an ensemble of larger models is defined as dark knowledge.
Intuitively, the knowledge is dark since the smaller network never had access to the training set of the larger one(s).

\subsection{Redefining Dark Knowledge}
\label{subsec:redefine_dark}
We extend or append to the dark knowledge definition by arguing that the darkness of knowledge should remain even if the disparity between the representational power of the teacher and the student network is exactly matched.
In simpler words, even if both networks were the same size, the teacher network's knowledge should be more informative and general.
In our context, this is ensured as the inputs to the teacher-student networks are different.
The teacher receives a more informative input, \textit{always}.
In our explicit knowledge distillation (dp-disparity-estimation) and implicit dark geometry teacher, the input to the teacher is the stereo-pair while the student has access only to the single dual pixel view.
Similarly, the flow teacher receives the next video sequence frame (2 images in a video sequence) however our student LF reconstruction model only uses the single dual pixel view again. 
See~\cref{fig:schematic_arch_dp_disparity} and~\cref{fig:full_arch}.
Also, temperature for us means the overall loss scalar multiplier instead of the conventional logit scalar in Hinton~\etal~\cite{kd_first_02}.

\subsection{Proposed Hypothesis}
We propose to distill dark stereo knowledge from a synthetically pretrained network to a tiny \textit{dp}-based network.
The intuitive goal is to learn RGB/dp channel dynamic switching or understand the camera's depth-of-field implicitly.

\subsection{Methodology}
Given a single dual pixel view $\{I_C, dp^C_L, dp^C_R\}$, the goal is to estimate a large-baseline (stereo) disparity using a tiny dp-network that is also mobile performant and understand when the dual pixel channels have defocus blur (or disparity information as formulated in~\cref{eq:dp_disparity_equation}) and when to rely solely on RGB channels. 
We allow the student network to freely optimize its latent space by using an explicit response-based distillation~\cite{response_01, response_02, response_03, response_04} technique like Hinton~\etal~\cite{kd_first_02}. This is to ensure that the camera depth-of-field or dynamic $RGB/dp$ channel switching can be learned. 
\begin{figure}[h]
    \centering
    \includegraphics[width=0.99\columnwidth]{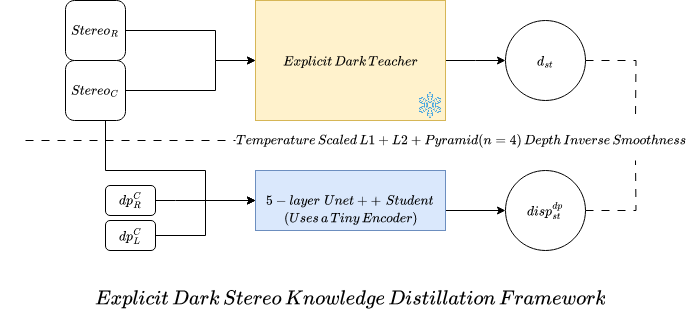}
    \caption{\textbf{Schematic Architecture} for our tiny-dp-disparity networks using the explicit version of dark knowledge distillation. See~\cref{subsec:redefine_dark} for the re-defined machine learning term: dark knowledge.}
    \label{fig:schematic_arch_dp_disparity}
\end{figure}

\begin{table*}[ht]
    \centering
    \caption{\textbf{Ablation: Efficiency vs. Accuracy of Dark-dp-Disparity Encoders}. Note that the GPU \& CPU wall times and parameters are for the full architecture and not just for the encoder. All GPU wall times are computed on an NVIDIA T4 GPU. We also train faster and more parametrically efficient models (R18 and Mv2-075) but their metrics were not computed by the paper-submission deadline.}
    \begin{tabular}{lccccc}
    \toprule
        \textbf{Encoders} & AI(1) $\downarrow$ & AI(2) $\downarrow$ & $W_{CPU}$ (ms) $\downarrow$ & $W_{GPU}$ (ms) $\downarrow$ & Params (M) $\downarrow$ \\
    \midrule
    ResNet18 & - & - & 478.129 & \textbf{8.244} & 15.97 \\ 
    ResNet34 & 0.129 & 0.169 & 538.26 & 11.20 & 26.08 \\ 
    ResNet50 & 0.129 & 0.165 & 1508.89 & 21.67 & 48.98 \\ 
    \midrule
    MobileNetv2 & 0.148  & 0.191 & 193.21 & 15.04 & 6.824 \\ 
    MobileNetv3-L75 & - & - & \textbf{162.19} & 17.42 & \textbf{5.078} \\ 
    MobileNetv3-L100 & 0.182  & 0.215 & 173.96 & 17.71 & 6.916 \\  
    \bottomrule
    \end{tabular}
    \label{tab:my_label_abl}
\end{table*}

Note that estimating a larger baseline disparity is possible as the network can theoretically learn to non-uniformly or locally stretch the dual pixel disparity $disp^{dp}_{st,x,y} = f_{\theta}(d^{dp}_{x,y})$ where $d^{dp}_{x,y}$ is the dual pixel disparity from~\cref{eq:dp_disparity_equation} while also relying on monocular context.
Monocular methods estimate depth and then inversely map it using the relation $Disp_{mono} = fZ_0 / \hat{z}$ where $f$ is the focal length, $Z_0$ is the maximum scene depth and $\hat{z}$ is the network's predicted depth.

\subsubsection{Architecture(s)}
We use a 5-layer deep U-Net++~\cite{unet_pp}, using the implementation provided by Pavel Iakubovskii~\cite{segModelsPytorch}, with four different off-the-shelf encoders, primarily geared for mobile and GPU performance.
The decoder has a single convolution layer appended, with no activation function thereafter, to output single channel disparity estimate of the desired resolution.
The encoders include residual networks~\cite{resnet} (Resnet-50 and Resnet-34) and mobile nets~\cite{mv} (Mobile Net v2~\cite{mv2} uses the inverted thin residual connections and Mobile Net v3-large~\cite{mv3} uses a Neural Architecture Search (NAS) technique to find the best model).
In our setup, the response comes from a synthetically pre-trained stereo teacher by Xu~\etal~\cite{xu2023unifying_unimatch} that distills its affine-invariant \textit{dark} knowledge or stereo disparity to the dual pixel network.

\subsubsection{Geometry-Teacher Selection}
Unimatch~\cite{xu2023unifying_unimatch} and STTR~\cite{STTR} were closely related work with the exact properties we wanted. However, to ensure the best results, at least on \textit{dp}MV, we \textit{qualitatively} evaluated both networks in addition to other cost-volume-based, feature matching, warping etc. stereo disparity estimators: IGEV~\cite{xu2023iterative_igev}, Graft-PSM~\cite{graft_psm_net}, ACVNet~\cite{xu2022attention_ACVNet} and CFNet~\cite{CF_Net_disp}.

We show the top-5, including hyper-parameter fine-tuned, performing teachers in~\cref{fig:teacher_selection}.

\subsubsection{Losses}
A weighted or temperature scaled (to stay consistent with knowledge distillation nomenclature) combination of $L1$, $L2$ and pyramid ($levels = n = 4$) depth inverse smoothness loss~\cite{monodepth17} is used that matches edges based on the gradients of the input RGB ($\partial_{Stereo_C}$).
Overall, the following loss is computed:

\begin{equation}
    \begin{aligned}
    L_{overall} = & T_1 \times \|d_{st}, disp^{dp}_{st}\|  + T_2 \times \|d_{st}, disp^{dp}_{st}\|_{2} + \\     
    &T_3 \times DISL(disp^{dp}_{st}, I_{C})
    \end{aligned}
    \label{eq:dp_disp_losses}
\end{equation}
where, $DISL$ is given by:
\begin{equation}
    \begin{aligned}
    DISL(disp^{dp}_{st}, I_{C}) = & \frac{1}{N}\sum_{i,j} {|\partial_{x}} disp^{dp}_{st,i,j}|e^{-\|{\partial_{x}} I_{C,x,y}\|} + \\    
    & |{\partial_{y}}disp^{dp}_{st,i,j}|e^{-\|{\partial_{y}} I_{C,x,y}\|}
    \end{aligned}
    \label{eq:depth_inverse_smoothness}
\end{equation}
where $I_{C,x,y}$ is the $(x,y)^{th}$ pixel of RGB input $Stereo_C$ and N is the total number of pixels or the resolution at the pyramid level.
The pyramid is built by bilinearly interpolating or downsizing by a factor of 2. 
So, the input resolution of $600\times 800$ is reduced to $\frac{600}{2^3} \times \frac{800}{2^3}$ on the top-most pyramid level.

\subsection{Implementation Details}
We train all models using PyTorch~\cite{pytorch} with the AdamW optimizer~\cite{adamW} using a learning rate of $3e-4$ and a Cosine Annealing Scheduler~\cite{scheduler} with $T_{max}=15$ and $eta_{min}=3e-6$.
All models are trained for an equal number of $50$ epochs on an $80-20$ leakage-free \textit{dp}MV split using a training batch size of 3 at an input resolution of $600 \times 800$ (the resolution at which the teacher outputs)
$T_1$, $T_2$ and $T_3$ are all set to 1.
% \begin{figure}[ht]
%     \centering
%     \includegraphics[width=0.9\columnwidth]{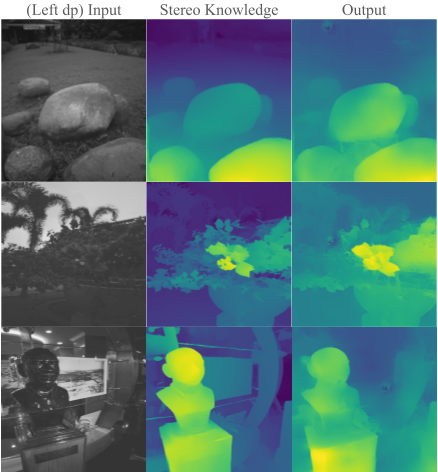}
%     \caption{More Qualitative Results from our best fidelity network (Dark-R50).}
%     \label{fig:dp_disp_more}
% \end{figure}

\subsection{Experiments}
In this section, we introduce the baselines, dataset, reference, and metrics for the quantitative benchmark and subsequent results \& limitations of our tiny-dp-disparity networks.

\subsubsection{Baselines}
\textbf{Monocular Disparity Estimation Baselines.}
We compare our tiny stereo knowledge distilled dual pixel-based disparity estimator, with 3 large state-of-the-art monocular depth estimation (MDE) methods.
It is possible to compare with MDEs as depth estimates ($Z$) are inversely proportional to disparity, dependent on the focal length ($f$) and maximum scene depth ($Z_0$) as follows: $d_{st} = f*Z_0 / Z$. 
Hence, all our MDE baselines operate under zero-shot \textit{metric} conditions instead of ambiguous scale, similar to ZoeDepth~\cite{zoeDepth}.
To that end, we compare with the latest Depth Anything~\cite{depth_anything}, DPT-Large~\cite{Ranftl2020}, and MiDaS~\cite{midas} monocular depth estimation converted to zero-shot metric conditions disparity baselines. 
% Write about each baseline. Hone down on efficiency: params and time. Also talk about training set sizes and compute required.
We demonstrate that a simple stereo-knowledge prior distilled to a tiny network utilizing dual pixels can outperform large, sophisticated, and massive compute using monocular depth estimators. 
Not using dual pixel views hinders the network's ability to find clear foreground-background separations resulting in smudged egdes~\cref{fig:qualitative}.

\textbf{Dual-Pixel based Disparity Estimation Baselines.}
We benchmark \textit{dp}MV with similar input (RGB+\textit{dp}) methods: DDDNet and DPDD
% Write briefly about each baseline & how our method compares
The rationale for choosing these MDE baselines with high representation power and massive training datasets is to demonstrate competitive or better disparity estimation fidelity while being \textit{practical} for deployment and downstream edge applications. 
Whereas, the main purpose for the \textit{dp}-baselines is to benchmark our \textit{dp}MV dataset and also provide a holistic comparison of the conventional disparity from dual pixel task.

\subsubsection{Evaluation Criteria}
\label{sec:affine_inv_metrics}       
We use affine invariant MAE ($AI(1)$) and affine invariant RMSE ($AI(2)$) for evaluation, similar to~\cite{punnappurath2020modeling}.
We also consider the number of parameters and the inference time to be significant factors for real-world use cases of such neural networks or kernel optimization-based methods.

\subsubsection{Quantitative Comparison and dpMV Benchmark}
All metrics are computed on a set of 145 images shown in~\cref{fig:all_dataset_IP_1},~\cref{fig:all_dataset_IP_2} and~\cref{fig:all_dataset_IP_3}.
The $CPU$ and $GPU$ runs are averaged on the same set, thrice for the GPU times and once for the CPU times.
Note that the times mentioned are per-image.
See~\cref{tab:benchmark_dpmv} for the quantitative benchmark on disparity estimation.

% \subsubsection{More Qualitative Results}
% See~\cref{fig:dp_disp_more}

\subsubsection{Ablation: Efficiency vs Accuracy}
In~\cref{tab:my_label_abl} we demonstrate the parameter and inference speed gains versus the drop in accuracy of our models. 

\subsubsection{Limitation. The Droplet Artifact due to Batch Normalization}
\label{sec:supp_batch_normalization}
Batch Normalization has been attributed to the water-droplet smudge artifact as first observed in styleGAN2~\cite{stylegan2} by Karras~\etal~\cite{stylegan3} (StyleGAN3).
Similarly, super-resolution methods like ESRGAN~\cite{esrgan} do not use batch normalization for any of the deep residual-in-residual blocks to maintain sharpness. 
\begin{figure}[h]
    \centering
    \includegraphics[width=0.99\columnwidth]{supp_imgs/dark_dp_est/limitation_styleGAN3.png}
    \caption{\textbf{Dark dp-disparity-networks' Limitation.} The water-droplet-like smudging that occurs for some estimations is attributed to the batch normalization layers in the decoder.}
    \label{fig:dark_dp_limitation}
\end{figure}
Similarly, we attribute this smudged or water-droplet effect in our dark-tiny-dp-disparity networks due to batch normalization layers in the decoder. 
\section{More Light Field Video Reconstruction}
\label{sec:lfvr_supplement}

\subsection{Properties in a Nutshell}
Here, we re-iterate the properties of our method concisely.

\textbf{Zero-shot Cross Dataset Transfer:}
Most existing literature requires fine-tuning on other datasets before evaluation, so we believe zero-shot cross-dataset transfer is an important generalization property for end-user applications.

\textbf{Zero-shot Inference of Higher (than training) Spatial-Angular Resolutions}
Our reconstructions remain geometrically consistent and our PSNR rises as the input spatial resolution increases. See figure 6 in main text and~\cref{tab:fig6_plot_values}.

\textbf{Implicit Disocclusion Handling}
We believe that if the feature extractor(s) understand the 3D scene well and have some context during training, they can learn to implicitly handle disocclusion by filling holes in extreme SAIs using the surroundings. 
Explicit hand-holding such as softmax-splatting~\cite{niklaus2020softmax} leads to a poorer 3D world understanding and often incorrectly splats foreground pixels to the background, see~\cref{sec:softmax_bad}.

\textbf{Fastest Inference and High Parameter Efficiency make our solution the most deployment fit to date.}
See the temporal consistency, parameters, and inference speed table in the main text.

\textbf{Highest Video LF Temporal Consistency.}
See \textit{supplementary slide 22} for video LF results.

\subsection{Full Model and Optimization Loop Figure}
The flow teacher $\flownet$ gets added after 100 training epochs with the geometry teacher. 
See~\cref{fig:full_arch} for a full model diagram alongside how the losses get distilled. The main text does not have the flow-teacher distillation loss schematic.

\begin{figure*}[ht]
    \centering
    \includegraphics[width=0.95\textwidth]{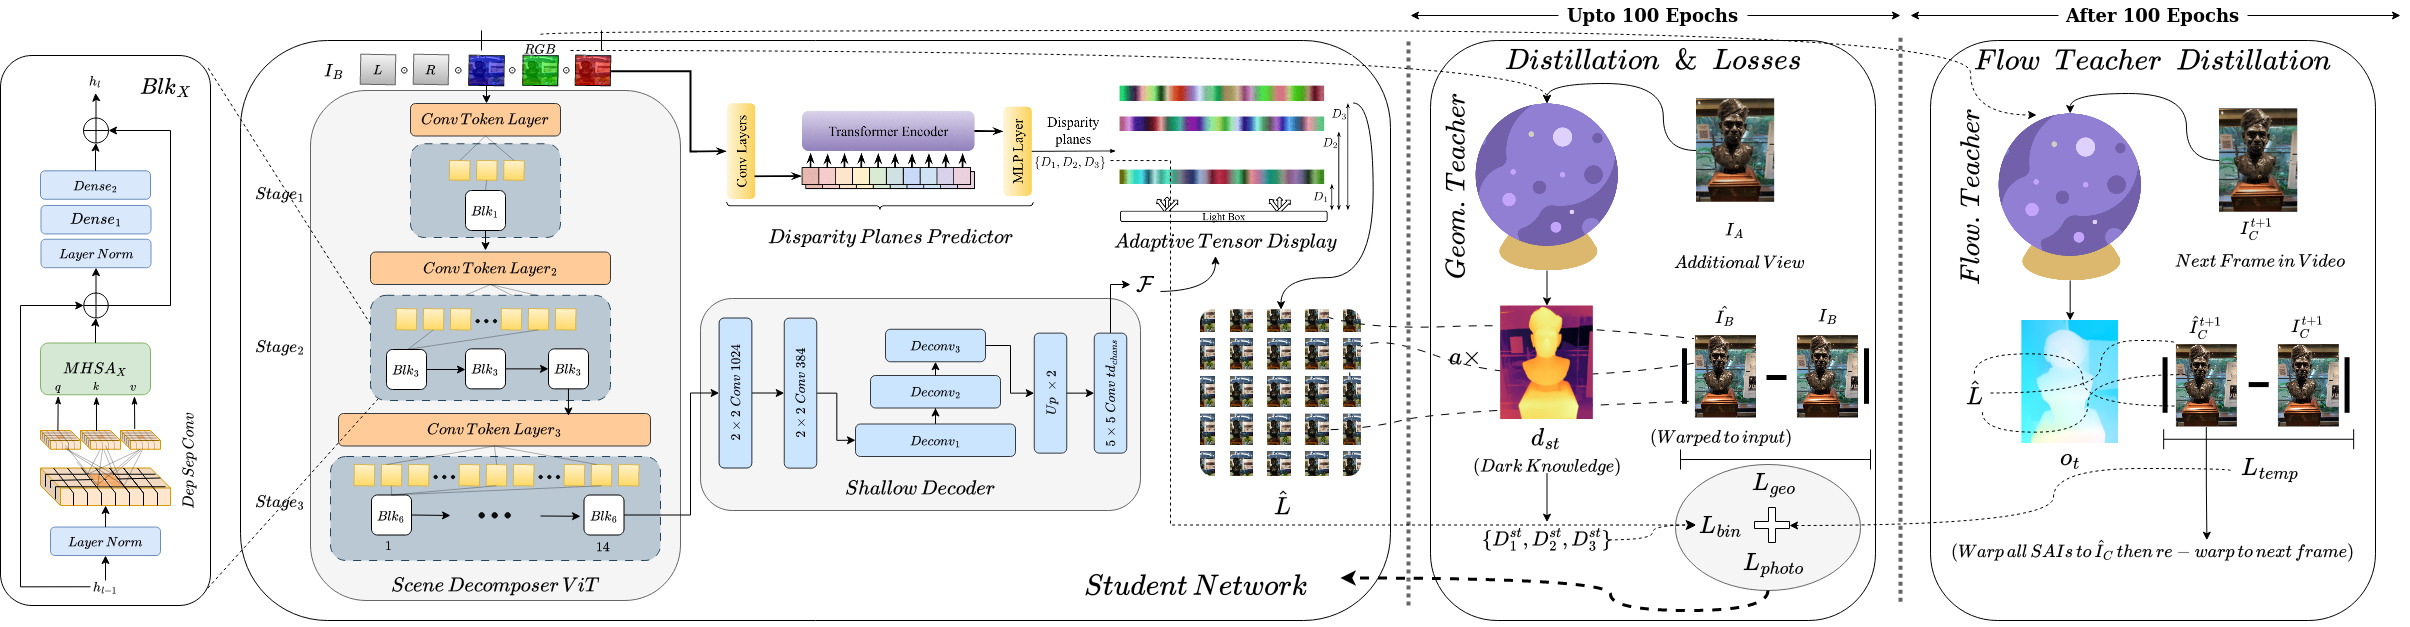}
    \caption{\textbf{Full Model Diagram with Losses.} Here, $\flownet$ takes the next video frame as input and computes an optical flow map $o_t$ using which all the warped-to-center SAIs ($\hat{I}_C$) are warped to the next video input frame, one by one.
The summation of the error gives the temporal loss.
Our method uses RAFT~\cite{raft_RAFT} as the flow-teacher ($\flownet$) and achieves the most temporally consistent video LFs.}
    \label{fig:full_arch}
\end{figure*}

\subsection{More Implementation Details}
% DeepSpeed's Zero-offloading-2~\cite{ren2021zerooffload} was initially explored but a simpler gradient accumulation of \textit{16-iterations} offered similar compute gains with a simpler training loop.
\textit{Extra losses tried.} D-SSIM~\cite{ssim} in conjunction with photometric loss. We discovered that it was not needed since the main scene decomposer could preserve global and local structure effectively so we chose to keep it simple. 
Additionally, we tried the softmax-splatting~\cite{niklaus2020softmax} formulation like Mono~\cite{eccv_22_monoLFVR} but only for boundary operating conditions of the dark knowledge scaling factor ($a > 3$).
The loss splatted foreground pixels to the background giving a sheared look to SAIs .

\subsection{Why explicit disocclusion handling or softmax-splatting~\cite{niklaus2020softmax} is inappropriate for LF reconstruction}
\label{sec:softmax_bad}
Softmax splatting~\cite{niklaus2020softmax} based disocclusion handling splats pixels, forcibly, from the foreground to the background. 
Notice how the ear stretches out as the baseline of generated LF increases in \textit{supplementary slide number 18} (Demonstration of the same phenomenon through GIFs).

\subsection{Simulating Dual Pixel Channels from Ground Truth Light Fields}
We average the adjacent SAI with the center view to get a dual-pixel channel. 
This works to an extent as the GT light fields do not have an adjacent SAI baseline $> 2$ pixels. 
Averaging naively brings the \textit{dp}-channel baseline to sub-pixel levels ($< 1$).
\begin{equation}
    dp_L = \frac{L(\mathbf{-1}) + L(\mathbf{0})}{2}
    \And
    dp_R = \frac{L(\mathbf{0}) + L(\mathbf{1})}{2}
\end{equation}
where $L(\mathbf{0})$ is the central view of the ground truth or captured Light Field(LF). $L(\mathbf{-1})$ and $L(\mathbf{1})$ correspond to the adjacent left and right sub-aperture views of the same LF.
See \textit{supplementary slide 20} for simulated dp-channels' GIF (sub-pixel baseline).

\subsection{Homography: To convert Image-LFs to Video-LFs for temporal consistency evaluation}
While we only require adjacent RGBs from a video sequence for the flow teacher that trains the LF student network to be temporally consistent; we require ground-truth $LF$ video to quantitatively evaluate the estimated $LF$ videos during the evaluation of temporal consistency.
For this, we generate $5$D $LF$ videos from a single $4$D $LF$ image.

Consider a $4$D $LF$ image of the form $L(x,y,u,v)$ where $(x,y)$ are the spatial co-ordinates and $(u,v)$ are the angular co-ordinates.
While simulating the video sequence, we assume a model of multiple pinhole cameras located at the co-ordinates $(u,v)$ from which individual views of the $LF$ are captured.
% Simulating a camera motion through the given light-field is equivalent to resampling the given $4$D light-field function and projecting it to the desired camera~\cite{lumentut2019fast,lfdeblurringlumentut}.
We consider the 6-DoF camera motion with translation and rotation defined as $P(t) = [\tx, \ty, \tz]$ and $R(t) = [\rx, \ry, \rz]$, respectively.
We consider the stereo camera located at the two views $(0,v_m)$ and $(U,v_m)$.
For the given 6-DoF translation and rotation $P(t)$ and $R(t)$ respectively, the left view at time $t$ is given by,
\begin{align}
    \leftframe &= L(x^j, y^j, p_x^i(t)-x^j\tz, v_m + p_y^i(t)-y^j\tz) \\
    x^j &= (x - U/2) \cos{\rz} - y \sin(\rz) + U/2 \\
    y^j &= (x - U/2) \sin{\rz} + y \cos(\rz) \\
    p_x^i&(t) = \tx + f\rx \\
    p_y^i&(t) = \ty + f\ry
\end{align}
where $f$ is the focal length of the camera.
Similarly, the right view of the camera is given by,
\begin{align}
    \rightframe = L(x^j, y^j, U + p_x^i(t)-x^j\tz, v_m + p_y^i(t)-y^j\tz)
    % x^j = (x - U/2) \cos{\rz} - y \sin(\rz) + U/2
    % y^j = (x - U/2) \sin{\rz} + y \cos(\rz) \\
    % p_x^i(t) = \tx + f\rx \\
    % p_x^i(t) = \ty + f\ry
\end{align}

% \subsection{Varying angular \& spatial resolution outputs}

\subsection{Quantitative Evaluation of Zero-Shotting Higher Spatial Resolutions than training}
In~\cref{tab:fig6_plot_values}, we report the exact values of the plot shown in Fig 6 (main text) that demonstrates how our method synthesizes geometrically consistent LFs even at very high, unseen, and modern-day required resolutions like close to Standard Definition ($480 \times 640$).

\begin{table}[ht]
    \centering
    \caption{\textbf{Zero-Shotting Higher Spatial Resolutions} - Quantitative Results (Fig 6 plot in main text)}
    \begin{tabular}{lcccccc}
        \toprule
        
        \textbf{Res.} & \cite{Niklaus_Ken_Burns} &  \textbf{Li} & \textbf{Li+}\cite{Ranftl2020} & \textbf{Mono} & \textbf{Mono-R} & \textbf{Ours}  \\
        
        \midrule
        $192^2$ & 20.564 & 26.285 & 25.730 & 26.369 & \textbf{26.622} & 25.754  \\  
        
        $256^2$ & 20.386 & 26.232 & 26.123 & 26.773 & \textbf{27.053} & 26.481 \\  
        
        $384^2$ & 16.574 & 26.056 & 26.033 &  26.748 & 27.023 & \textbf{27.082 } \\  
        
        $480^2$ & 16.444 & 25.928 & 25.926 & 26.791 & 27.249  & \textbf{27.304}  \\  
        % \midrule
        \bottomrule
    \end{tabular}
    \label{tab:fig6_plot_values}
\end{table}

\begin{figure}[ht]
    \centering
    \includegraphics[width=0.99\columnwidth]{supp_imgs/lfvr/epi_SD_1.5x.png}
    \caption{\textbf{Geometrically Consistent EPIs at Higher (Zero Shot) Spatial Resolutions} with the LF baseline, dark knowledge scaling hyperparameter ($a = 1.5$) larger than GT LF baselines.}
    \label{fig:ZS_higher_res}
\end{figure}

\begin{figure}[ht]
    \centering
    \includegraphics[width=0.6\columnwidth]{supp_imgs/lfvr/extreme_a_4.png}
    \caption{\textbf{Limitaion. Extremely Large Dark Knowledge Scaling Factor.} $a = 4$ produces artifacts around foreground-background separation regions in extreme sub-aperture images (SAIs) }
    \label{fig:limitation_1}
\end{figure}

\subsection{Qualitative Evaluation of Zero-Shotting Higher Spatial Resolutions - Geometrically Consistent EPIs}
Our method achieves geometric, Consistent epipolar images (EPIs) at Standard Definition ($480 \times 640$).
% \begin{figure*}[ht]
%     \centering
%     \includegraphics[width=0.99\textwidth]{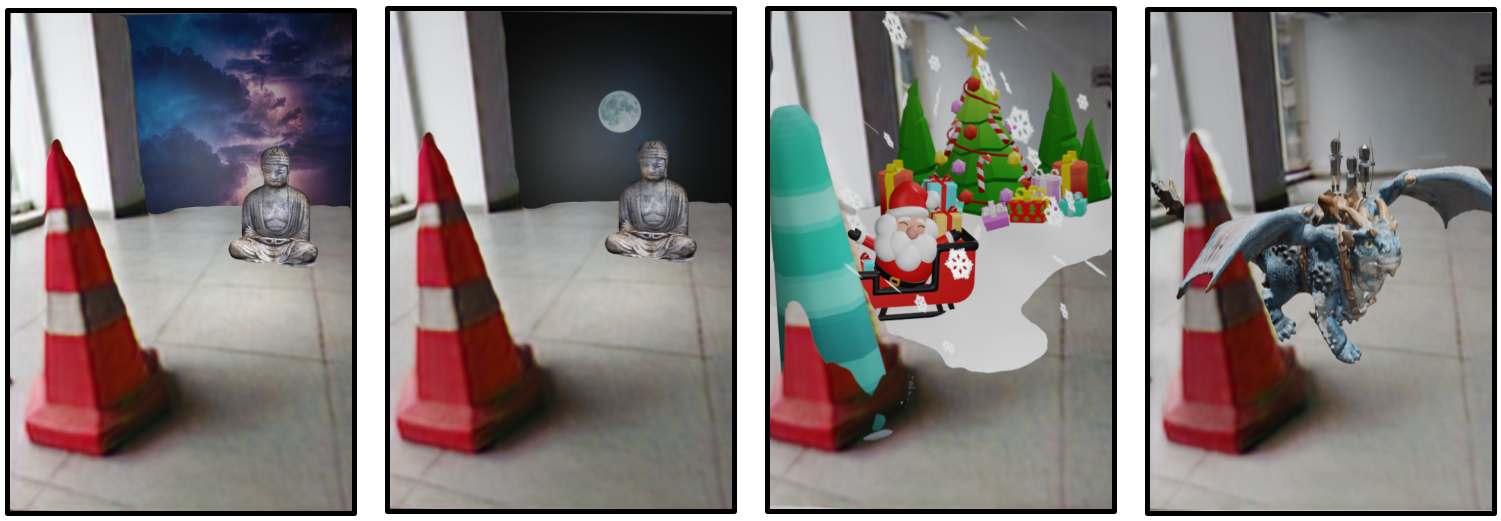}
%     \caption{\textbf{XR Applications} of Our Reconstructed Light Fields.}
%     \label{fig:xr_applications}
% \end{figure*}

\subsection{More Applications - Refocusing \& Novel View Synthesis}
Refocusing is shown in~\cref{fig:refocus}.
Novel view synthesis crops are shown in~\cref{fig:nvs_all}.

\begin{figure}[ht]
    \centering
    \begin{subfigure}{0.46\textwidth}
        \includegraphics[width=\textwidth]{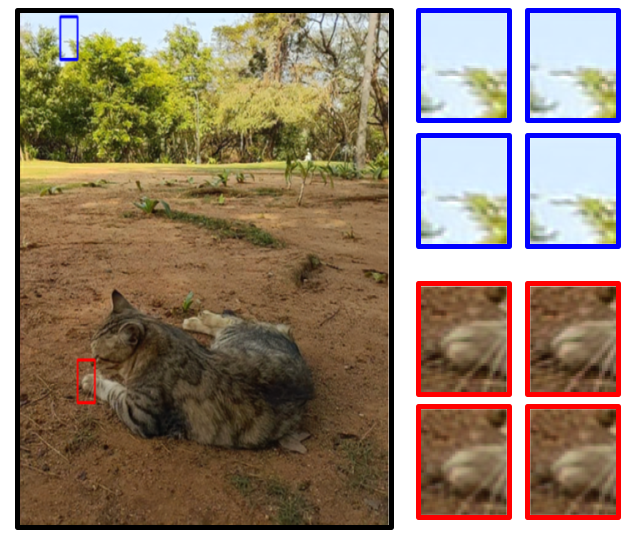}
    \end{subfigure}
    \hfill
    \centering
    \begin{subfigure}{0.46\textwidth}
        \includegraphics[width=\textwidth]{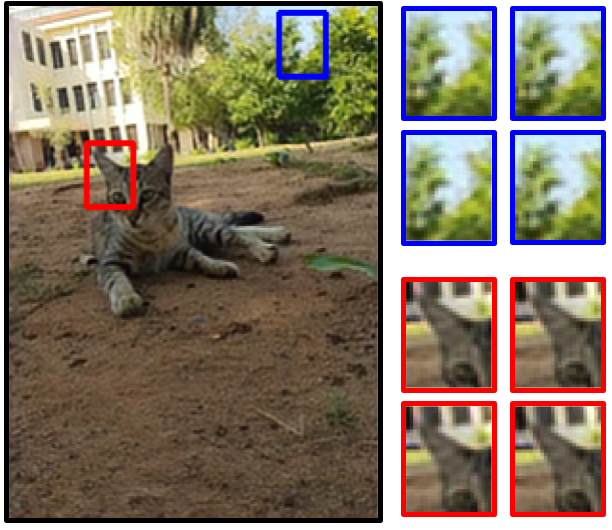}
    \end{subfigure}
    \caption{\textbf{Novel View Synthesis} using reconstructed Light Fields. The shift in crops exists as they are extreme Top-Left, top-right, bottom-left, and bottom-right SAIs of the LF respectively.}
    \label{fig:nvs_all}
\end{figure}

\subsection{Limitation 1 - Extreme Dark Knowledge Scaling} 
The failure mode occurs due to stretching our dark knowledge disparity estimate ($d_{st}$) too much.
This phenomenon is observed for values of $a > 3$.
Extreme SAIs suffer due to ineffective dual pixel guidance as the uneven stretching of dark knowledge becomes more prominent, see~\cref{fig:limitation_1}

\subsection{Limitation 2 - Extremely Transmissive and Reflective Surfaces}
Our method is not designed to reconstruct transmissive and extremely reflective surfaces.
\textit{dp}MV has a few such scenes shown in~\cref{fig:transmissive_reflective} and~\cref{fig:hardest_scene}.
Flickering artifacts can also be seen in reconstructed LFs for extremely shiny or non-Lambertian scenes.

% \subsection{Extreme Values of Dark Knowledge Scaling Hyper-parameter}
\section{\textit{dp}MV Dataset} 
\label{sec:dataset}
\begin{figure}[h]
    \centering
    \includegraphics[width=0.99\columnwidth]{supp_imgs/dataset/dataset_rig.png}
    \caption{\textbf{Dataset Capturing Rig:} Front and Back.}
    \label{fig:front_back_rig}
\end{figure}
\begin{figure}[h]
    \centering
    \includegraphics[width=0.9\columnwidth]{supp_imgs/dataset/fpsvsthreads.jpg}
    \caption{Maximum Capture $fps$ versus number of threads}
    \label{fig:capture_fps_number_of_threads}
\end{figure}

In this section, we highlight the categorized and annotated scenes and follow up by providing more details of the capturing, synchronization and storing procedure.

\subsection{Hardest Scene of dpMV}
\label{subsec:hardest_scene}
This scene contains extremely non-Lambertian surfaces, and reflective \& transmissive glass panels simultaneously.

\begin{figure}[ht]
    \centering
    \includegraphics[width=0.9\columnwidth]{supp_imgs/dataset/hardest_scene.png}
    \caption{\textbf{Hardest Transmissive, Reflective and Non-Lambertian Scene in \textit{dp}MV.} Even the dark stereo geometry teacher's disparity estimate ($d_{st}$) is \textit{poor} quality and untrue to the scene. 
    We never use this scene for training or testing purposes.
    }
    \label{fig:hardest_scene}
\end{figure}
\subsection{Transmissive, Reflective and Non-Lambertian Scenes}
Our methods are not designed for these scenes but we hope that the reflective-transmissive surface reconstruction community finds these scenes useful.

\subsection{Scene Categories} 
\textbf{One representative image for each scene (video) with the classification category is shown in~\cref{fig:all_dataset_IP_1},~\cref{fig:all_dataset_IP_2} and~\cref{fig:all_dataset_IP_3}.}
We consider the category as the 1-or-2-word caption of the entire video.

\subsection{Capturing Rig}
We show the front and back of our rig in~\cref{fig:front_back_rig}.

\subsection{Synchronization}
To synchronize capture across three devices, Simple Network Time Protocol (SNTP) is utilized. Phones obtain offsets from a public NTP server. A designated device acts as the master, determining the start time for capture across all devices. The master's chosen timestamp is sent to a web server, and other devices fetch this adjusted target timestamp to initiate capture simultaneously. To validate synchronization, we record a timer before capture and manually adjust frames post-capture if synchronization issues arise.

\subsection{Capture Frame Rate}
To optimize our capture process, an optimal frame rate is crucial. If the frame rate is too high, frame synchronization becomes challenging. The total time per frame involves both I/O time for storing the frame and processing time, including dual pixel quantization to 8 bits and JPEG compression~\cite{GargDualPixelsICCV2019_DPNet}. Processing multiple frames in parallel reduces processing time, thus increasing the supported frame rate. Empirically, using around 6 worker threads achieves the best performance, consistently reaching approximately 18 FPS without frame drops. However, performance decreases at higher CPU temperatures. Given that much of our dataset is captured outdoors with elevated temperatures, we capped the actual capture frame rate at 13 $fps$ (see~\cref{fig:capture_fps_number_of_threads}).

\subsection{Processing \textit{dp}-Frames}
The Pixel-4 phones provide dual pixel data at 10-bit resolution which are re-quantized to 8 bits and stored with JPEG compression. We minimize quantization loss similar to \cite{GargDualPixelsICCV2019_DPNet} by first re-scaling the data to $0-2^{16}$ and then compressing to 8-bit integer depth followed by quantization.

\begin{figure*}[ht]
    \centering
    \begin{subfigure}{0.9\textwidth}
        \includegraphics[width=\textwidth]{supp_imgs/dataset/nl_scenes_1.png}
    \end{subfigure}
    \hfill
    \begin{subfigure}{0.9\textwidth}
        \centering
        \includegraphics[width=0.7\textwidth]{supp_imgs/dataset/nl_scenes_2.png}
    \end{subfigure}
    \caption{\textbf{Transmissive, Reflective and Non-Lambertian Scenes of \textit{dp}MV.} The top row shows harder scenes compared to the bottom two. The last row predominantly focuses on visible light sources.}
    \label{fig:transmissive_reflective}
\end{figure*}

\section{Discussion}
\label{sec:discussion}
Through this supplementary, we have extended the motivation of our work and validated our direction \textit{with theory} to reach a hypothesis beneficial for dual-pixel solutions.
The hypothesis is elaborated upon and finally validated as we report the \textit{dp}MV benchmark, qualitative results, ablations, and comparisons on the dual-pixel disparity estimation comprehensively. We also provide our methodology, implementation details, and schematics for the same.
To further test the effectiveness of our dark knowledge hypothesis, we demonstrate a single-view light field video reconstruction method. 
In the process, we push the light field research forward by using dual pixels, showing the use of vision transformers for the first time and achieving the fastest and most temporally consistent light field videos. 
We provide the theory for simulating our dual pixel channels and homographic transforms. 
We show additional results, and experiments, discuss the appropriateness of softmax splatting for explicit disocclusion handling, and end the section with a demonstration of our method.
Finally, we show our dataset in detail with the categorized and captioned form in which it exists and will be released.

\begin{figure*}[htb!]
    \centering
    \begin{subfigure}{0.9\textwidth}
        \includegraphics[width=\textwidth]{supp_imgs/dataset/samples_1.png}
    \end{subfigure}
    \hfill
    \begin{subfigure}{0.9\textwidth}
        \includegraphics[width=\textwidth]{supp_imgs/dataset/samples_2.png}
    \end{subfigure}
    \caption{\textbf{\textit{dp}MV scenes - 1/3.} Except the hardest one shown in~\cref{subsec:hardest_scene}.}
    \label{fig:all_dataset_IP_1}
\end{figure*}

\begin{figure*}[hbt!]
    \centering
    \begin{subfigure}{0.9\textwidth}
        \includegraphics[width=\textwidth]{supp_imgs/dataset/samples_4.png}
    \end{subfigure}
    \hfill
    \begin{subfigure}{0.9\textwidth}
        \includegraphics[width=\textwidth]{supp_imgs/dataset/samples_5.png}
    \end{subfigure}
    \caption{\textbf{\textit{dp}MV scenes - 2/3.} Except the hardest one shown in~\cref{subsec:hardest_scene}.}
    \label{fig:all_dataset_IP_2}
\end{figure*}

\begin{figure*}[hbt!]
    \centering
    \begin{subfigure}{0.9\textwidth}
        \includegraphics[width=\textwidth]{supp_imgs/dataset/samples_3.png}
    \end{subfigure}
    \hfill
    \begin{subfigure}{0.9\textwidth}
        \includegraphics[width=\textwidth]{supp_imgs/dataset/samples_6.png}
    \end{subfigure}
    \caption{\textbf{\textit{dp}MV scenes - 3/3.} Except the hardest one shown in~\cref{subsec:hardest_scene}.}
    \label{fig:all_dataset_IP_3}
\end{figure*}

\clearpage
