# Supplementary material for: Stereo-Knowledge Distillation from dpMV to Dual Pixels for Light Field Video Reconstruction
Source: arXiv:2405.11823 source file (2024-05-20)
Supplement: Supplementary file 2 [file contrib.tex]

\section{Contributions}
\label{sec:contributions}
Overall, we contribute a central distillation idea for the computational imaging field, 4+1 \textit{dp}-models that perform camera depth-of-field aware disparity estimation and light field video reconstruction, using the distillation hypothesis, and a first-of-its-kind large dual pixel multi-view videos (\textit{dp}MV) dataset.

\subsection{Novelty.}
\begin{enumerate}
    \item \textit{Central Hypothesis of the paper.} Dark Knowledge distillation, implicit or explicit, from synthetically pre-trained stereo methods to dual pixel networks.
    
    \item \textit{dpMV dataset} to push methods using our hypothesis and other dual pixel and multi-view tasks including classification, captioning and multi-modal learning as the dataset comes with classes and 1-to-2 word captions as well.
    
    \item Validation of the hypothesis on disparity estimation task while \textit{benchmarking} dpMV. Here, 4 dark-dp-disparity networks are contributed.
    
    \item An application of the implicit version of the hypothesis is demonstrated for \textit{single dp-view light field video reconstruction}, for the first time.

    \item The first use case of vision transformers for light field reconstruction.

    \item LF reconstruction achieves the lowest inference time while maintaining the highest video temporal consistency.
\end{enumerate}

% b) The \textbf{58,295 frames' dual-pixel video dataset captured in dynamic environments. The dataset also has additional rectified \& synchronized stereoscopic views}. 
% The multi-view dataset enables conventional vision tasks in addition to providing researchers the opportunity to solve the same tasks with the ubiquitous dual-pixels (found in most smartphones nowadays) using \textbf{the cross-modal pretext (additional views), thus encouraging self-supervised research}.  
% \textbf{b) We contribute the first method for LF reconstruction using dual pixels}. 

% c) We also show \textbf{the first use case of vision transformers (ViT) for LF reconstruction}. 
% The zero-shot cross-data, angular \& spatial characteristics, while being competitive with the prior refinement-based supervised methods and state-of-the-art without supervision, demonstrate the superiority of our novel architectural choice, design, and training setup. 
% These choices were based on the \textbf{key insight} that the dual pixels could provide implicit disparity cues essential for LF reconstruction while also finely guiding the network along tricky edges (See Figure 6).  

% d) Our method also has the \textbf{lowest inference time and requires no extra inputs unlike most LF methods}.

\subsection{Significant Differences \& Advantages over Monocular and Stereo Light Field State-of-the-Art Methods}
While our work shares some similarities with Mono~\cite{eccv_22_monoLFVR} and SelFVi~\cite{Selfvi}, significant differences distinguish our approach, leading to substantial improvements over these methods.
To name a few, generalization or zero-shot properties, speed, parameter efficiency, no extra hardware calibration, no post-processing costs, no external network dependencies, and no need for ground truth light fields for refinement are some crucial gains arising from our method.
On a deeper level, our approach solves the hardest task of truly understanding the 3D scene while being hardware-practical:

\textbf{Difficulty of task.}
SeLFVi computes disparity from its stereo input explicitly unlike our implicit methods for computing the disparity plane centers. 
While we predict disparity planes using just the dual pixel input, Mono relies on explicit disparity estimates as input from an external pretrained DPT-384-Large~\cite{Ranftl2020}).
This provides Mono's network explicit 3D context and never is encouraged to capture the critical question "What does the 3D world look like" (Input Ablation Table and Input Ablation Breakdown section in the main text).
Our method is encouraged to do so through the distillation losses.

\textbf{Difficulty of Geometric Consistency.}
SeLFVi has to reconstruct one less sub-aperture view while also getting a better geometric consistency loss as the left view becomes the left-most SAI while the right view becomes the center SAI of the predicted light field for their method. 
Our method only has the central view but not the explicit disparity input (like Mono). 
Mono learns a simple pixel re-arrangement relation using the RGB + disparity input used during inference. 
For ours, a true 3D scene understanding is essential for correct SAI reconstruction (warping and hole-filling from single view) during inference.

\textbf{Ease of and load on hardware.}
Our exclusive use of RGP+DP channels eliminates smartphone deployment impracticalities for stereo cameras. 
Our ViT-based model has state-of-the-art inference times (Table 4) and is extremely parameter efficient with generalization capabilities across different types of datasets (or scenes) and user-defined settings like LF spatial-angular resolution, and baseline. 
Mono is resource-consuming, and impractical for user applications, especially due to the external massive depth-network \textit{required} during inference. 
Also, Mono does not generalize across datasets without the refinement module (fully supervised on GT LFs).

\textbf{Appropriateness of Vision Transformers for (dense) light field reconstruction} 
The synergy of dual pixels and ViT enables us to streamline reconstruction without explicit disocclusion handling, providing an efficient 3D scene understanding. 
The dual pixels play a guiding role in the reconstruction along edges (Fig. 6) and also provide imperative disparity cues without which the model never converges due to limited representational power and compute resources (Input side ablation Table in main paper). 

\subsection{Note on Cross-Modal Self-Supervision Taxonomy}
According to Jaiswal~\etal~\cite{rebuttal_01}, our method falls under cross-modal-pretext self-supervised learning (SSL) tasks, defined therein as follows: "Pretext tasks are self-supervised tasks that act as an important strategy to learn representations of the data using pseudo labels. These pseudo labels are generated automatically based on the attributes found in the data." 
Cross-modal is the additional view $I_A$ used to compute a stereo disparity estimate ($d_{st}$) or the pseudo-label computed from attributes ($I_A$) found in the dataset. 
Rani~\etal~\cite{rebuttal_02} uses the same operational definition by using a task-level classification: auxiliary pretext tasks and pseudo labels therein. 
Also, we never captured or had access to ground truth light fields to begin with so it rules out semi-supervised or weakly-supervised regimes that rely on partially labeled (GT) data to make sense of the unlabelled data during training.
