# Supplementary material for: Stereo-Knowledge Distillation from dpMV to Dual Pixels for Light Field Video Reconstruction
Source: arXiv:2405.11823 source file (2024-05-20)
Supplement: Supplementary file 3 [file dark.tex]

\section{Dark Knowledge Distillation to dp-Disparity Networks}
\label{sec:dark}

% \begin{figure*}[h]
%     \centering
%     \includegraphics[width=0.9\textwidth]{supp_imgs/dark_dp_est/geometry_teacher_comparison.png}
%     \caption{\textbf{Dark Knowledge Stereo Disparity Teacher Selection.} $FT$ stands for hyper-parameter fine-tuned. 
%     Note that ACVNet~\cite{xu2022attention_ACVNet} and STTR~\cite{STTR} were also tried on the scenes of \textit{dp}MV but performed poorer than the shown methods.
%     The stereo teacher selected here is also used as the geometry teacher for our light field video reconstruction method (\cref{sec:lfvr_supplement})}
%     \label{fig:teacher_selection}
% \end{figure*}

\begin{table*}[ht]
    \caption{\textbf{Quantitative Comparison and \textit{dp}MV Benchmark} with Our Dark \textit{dp}-Disparity Estimators. 
    All Wall clock times ($W_{GPU}$ and $W_{CPU}$), per estimation, are in mili-seconds measured on a single NVIDIA RTX 3090.
    Parameters ($Params$) are in millions. 
    Even though MiDaS is significantly smaller and faster than DPT-Large-384, it is prone to a massive fidelity drop of close to $76\%$ compared to the same.}
    \centering
    \begin{tabular}{lccccccc}
    \toprule
    % Choose best metrics (left our rn: log-RMSE, Sq_Rel, \del < 1.25^2)
        Method & AI(1) & AI(2) & Params  & $W_{CPU}$ & $W_{GPU}$  \\
        \midrule \midrule
        Depth-Anything~\cite{depth_anything} & 0.212 & 0.261 & 335.3 & $>$20000 & 72.38 \\     
        DPT-Large~\cite{Ranftl2020} & 0.196 & 0.231 & 344.05 & 11770.71 & 17.63 \\  
        MiDaS~\cite{midas} & 0.237 & 0.304 & 21.32 & 427.31 & 13.82 \\     
        \midrule  
        DDDNet~\cite{Pan_2021_CVPR_DDDNet_DP_Disp} & 0.298 & 0.389  &  10.964  & 4223.05 & 73.34 \\    
        DPDD~\cite{punnappurath2020modeling} & 0.221 & 0.341 & - & $>$20000 & - \\  
        \midrule
        \textbf{Ours-Mv2} & 0.148 & 0.191 & \textbf{6.824} & 193.21 & 15.04 \\
        \textbf{Ours-Mv3-CPU}  & 0.182 & 0.215 & 6.916  & \textbf{173.96} & 17.71 &  \\ 
        \midrule
        \textbf{Ours-R34-{GPU}} & 0.129 & 0.169 &  26.08 & 538.26 & \textbf{11.20} \\
        \textbf{Ours-R50-Best} & \textbf{0.129} & \textbf{0.165}  & 48.98 & 1508.89 & 21.67 \\ 
    \bottomrule
    \end{tabular}
    \label{tab:benchmark_dpmv}
\end{table*}

\subsection{What is Dark Knowledge?}
Rich Caruana~\etal~\cite{kd_first_01} showed how to \textit{distill} knowledge from an ensemble of large models to a small or compressed model.
Subsequently, Geoffrey Hinton~\etal~\cite{kd_first_02} argued that transferring knowledge from a large general yet cumbersome model to a smaller network using \textit{temperature raised soft logits} (in classification task context) enables better smaller model performance. 
This temperature-scaled output from the larger model or an ensemble of larger models is defined as dark knowledge.
Intuitively, the knowledge is dark since the smaller network never had access to the training set of the larger one(s).

\subsection{Redefining Dark Knowledge}
\label{subsec:redefine_dark}
We extend or append to the dark knowledge definition by arguing that the darkness of knowledge should remain even if the disparity between the representational power of the teacher and the student network is exactly matched.
In simpler words, even if both networks were the same size, the teacher network's knowledge should be more informative and general.
In our context, this is ensured as the inputs to the teacher-student networks are different.
The teacher receives a more informative input, \textit{always}.
In our explicit knowledge distillation (dp-disparity-estimation) and implicit dark geometry teacher, the input to the teacher is the stereo-pair while the student has access only to the single dual pixel view.
Similarly, the flow teacher receives the next video sequence frame (2 images in a video sequence) however our student LF reconstruction model only uses the single dual pixel view again. 
See~\cref{fig:schematic_arch_dp_disparity} and~\cref{fig:full_arch}.
Also, temperature for us means the overall loss scalar multiplier instead of the conventional logit scalar in Hinton~\etal~\cite{kd_first_02}.

\subsection{Proposed Hypothesis}
We propose to distill dark stereo knowledge from a synthetically pretrained network to a tiny \textit{dp}-based network.
The intuitive goal is to learn RGB/dp channel dynamic switching or understand the camera's depth-of-field implicitly.

\subsection{Methodology}
Given a single dual pixel view $\{I_C, dp^C_L, dp^C_R\}$, the goal is to estimate a large-baseline (stereo) disparity using a tiny dp-network that is also mobile performant and understand when the dual pixel channels have defocus blur (or disparity information as formulated in~\cref{eq:dp_disparity_equation}) and when to rely solely on RGB channels. 
We allow the student network to freely optimize its latent space by using an explicit response-based distillation~\cite{response_01, response_02, response_03, response_04} technique like Hinton~\etal~\cite{kd_first_02}. This is to ensure that the camera depth-of-field or dynamic $RGB/dp$ channel switching can be learned. 
\begin{figure}[h]
    \centering
    \includegraphics[width=0.99\columnwidth]{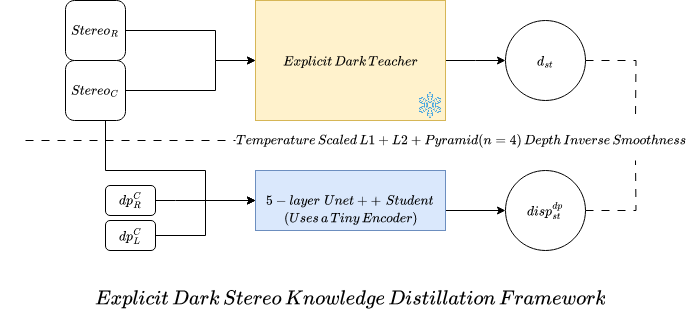}
    \caption{\textbf{Schematic Architecture} for our tiny-dp-disparity networks using the explicit version of dark knowledge distillation. See~\cref{subsec:redefine_dark} for the re-defined machine learning term: dark knowledge.}
    \label{fig:schematic_arch_dp_disparity}
\end{figure}

\begin{table*}[ht]
    \centering
    \caption{\textbf{Ablation: Efficiency vs. Accuracy of Dark-dp-Disparity Encoders}. Note that the GPU \& CPU wall times and parameters are for the full architecture and not just for the encoder. All GPU wall times are computed on an NVIDIA T4 GPU. We also train faster and more parametrically efficient models (R18 and Mv2-075) but their metrics were not computed by the paper-submission deadline.}
    \begin{tabular}{lccccc}
    \toprule
        \textbf{Encoders} & AI(1) $\downarrow$ & AI(2) $\downarrow$ & $W_{CPU}$ (ms) $\downarrow$ & $W_{GPU}$ (ms) $\downarrow$ & Params (M) $\downarrow$ \\
    \midrule
    ResNet18 & - & - & 478.129 & \textbf{8.244} & 15.97 \\ 
    ResNet34 & 0.129 & 0.169 & 538.26 & 11.20 & 26.08 \\ 
    ResNet50 & 0.129 & 0.165 & 1508.89 & 21.67 & 48.98 \\ 
    \midrule
    MobileNetv2 & 0.148  & 0.191 & 193.21 & 15.04 & 6.824 \\ 
    MobileNetv3-L75 & - & - & \textbf{162.19} & 17.42 & \textbf{5.078} \\ 
    MobileNetv3-L100 & 0.182  & 0.215 & 173.96 & 17.71 & 6.916 \\  
    \bottomrule
    \end{tabular}
    \label{tab:my_label_abl}
\end{table*}

Note that estimating a larger baseline disparity is possible as the network can theoretically learn to non-uniformly or locally stretch the dual pixel disparity $disp^{dp}_{st,x,y} = f_{\theta}(d^{dp}_{x,y})$ where $d^{dp}_{x,y}$ is the dual pixel disparity from~\cref{eq:dp_disparity_equation} while also relying on monocular context.
Monocular methods estimate depth and then inversely map it using the relation $Disp_{mono} = fZ_0 / \hat{z}$ where $f$ is the focal length, $Z_0$ is the maximum scene depth and $\hat{z}$ is the network's predicted depth.

\subsubsection{Architecture(s)}
We use a 5-layer deep U-Net++~\cite{unet_pp}, using the implementation provided by Pavel Iakubovskii~\cite{segModelsPytorch}, with four different off-the-shelf encoders, primarily geared for mobile and GPU performance.
The decoder has a single convolution layer appended, with no activation function thereafter, to output single channel disparity estimate of the desired resolution.
The encoders include residual networks~\cite{resnet} (Resnet-50 and Resnet-34) and mobile nets~\cite{mv} (Mobile Net v2~\cite{mv2} uses the inverted thin residual connections and Mobile Net v3-large~\cite{mv3} uses a Neural Architecture Search (NAS) technique to find the best model).
In our setup, the response comes from a synthetically pre-trained stereo teacher by Xu~\etal~\cite{xu2023unifying_unimatch} that distills its affine-invariant \textit{dark} knowledge or stereo disparity to the dual pixel network.

\subsubsection{Geometry-Teacher Selection}
Unimatch~\cite{xu2023unifying_unimatch} and STTR~\cite{STTR} were closely related work with the exact properties we wanted. However, to ensure the best results, at least on \textit{dp}MV, we \textit{qualitatively} evaluated both networks in addition to other cost-volume-based, feature matching, warping etc. stereo disparity estimators: IGEV~\cite{xu2023iterative_igev}, Graft-PSM~\cite{graft_psm_net}, ACVNet~\cite{xu2022attention_ACVNet} and CFNet~\cite{CF_Net_disp}.

We show the top-5, including hyper-parameter fine-tuned, performing teachers in~\cref{fig:teacher_selection}.

\subsubsection{Losses}
A weighted or temperature scaled (to stay consistent with knowledge distillation nomenclature) combination of $L1$, $L2$ and pyramid ($levels = n = 4$) depth inverse smoothness loss~\cite{monodepth17} is used that matches edges based on the gradients of the input RGB ($\partial_{Stereo_C}$).
Overall, the following loss is computed:

\begin{equation}
    \begin{aligned}
    L_{overall} = & T_1 \times \|d_{st}, disp^{dp}_{st}\|  + T_2 \times \|d_{st}, disp^{dp}_{st}\|_{2} + \\     
    &T_3 \times DISL(disp^{dp}_{st}, I_{C})
    \end{aligned}
    \label{eq:dp_disp_losses}
\end{equation}
where, $DISL$ is given by:
\begin{equation}
    \begin{aligned}
    DISL(disp^{dp}_{st}, I_{C}) = & \frac{1}{N}\sum_{i,j} {|\partial_{x}} disp^{dp}_{st,i,j}|e^{-\|{\partial_{x}} I_{C,x,y}\|} + \\    
    & |{\partial_{y}}disp^{dp}_{st,i,j}|e^{-\|{\partial_{y}} I_{C,x,y}\|}
    \end{aligned}
    \label{eq:depth_inverse_smoothness}
\end{equation}
where $I_{C,x,y}$ is the $(x,y)^{th}$ pixel of RGB input $Stereo_C$ and N is the total number of pixels or the resolution at the pyramid level.
The pyramid is built by bilinearly interpolating or downsizing by a factor of 2. 
So, the input resolution of $600\times 800$ is reduced to $\frac{600}{2^3} \times \frac{800}{2^3}$ on the top-most pyramid level.

\subsection{Implementation Details}
We train all models using PyTorch~\cite{pytorch} with the AdamW optimizer~\cite{adamW} using a learning rate of $3e-4$ and a Cosine Annealing Scheduler~\cite{scheduler} with $T_{max}=15$ and $eta_{min}=3e-6$.
All models are trained for an equal number of $50$ epochs on an $80-20$ leakage-free \textit{dp}MV split using a training batch size of 3 at an input resolution of $600 \times 800$ (the resolution at which the teacher outputs)
$T_1$, $T_2$ and $T_3$ are all set to 1.
% \begin{figure}[ht]
%     \centering
%     \includegraphics[width=0.9\columnwidth]{supp_imgs/dark_dp_est/dp_est_qual_more.png}
%     \caption{More Qualitative Results from our best fidelity network (Dark-R50).}
%     \label{fig:dp_disp_more}
% \end{figure}

\subsection{Experiments}
In this section, we introduce the baselines, dataset, reference, and metrics for the quantitative benchmark and subsequent results \& limitations of our tiny-dp-disparity networks.

\subsubsection{Baselines}
\textbf{Monocular Disparity Estimation Baselines.}
We compare our tiny stereo knowledge distilled dual pixel-based disparity estimator, with 3 large state-of-the-art monocular depth estimation (MDE) methods.
It is possible to compare with MDEs as depth estimates ($Z$) are inversely proportional to disparity, dependent on the focal length ($f$) and maximum scene depth ($Z_0$) as follows: $d_{st} = f*Z_0 / Z$. 
Hence, all our MDE baselines operate under zero-shot \textit{metric} conditions instead of ambiguous scale, similar to ZoeDepth~\cite{zoeDepth}.
To that end, we compare with the latest Depth Anything~\cite{depth_anything}, DPT-Large~\cite{Ranftl2020}, and MiDaS~\cite{midas} monocular depth estimation converted to zero-shot metric conditions disparity baselines. 
% Write about each baseline. Hone down on efficiency: params and time. Also talk about training set sizes and compute required.
We demonstrate that a simple stereo-knowledge prior distilled to a tiny network utilizing dual pixels can outperform large, sophisticated, and massive compute using monocular depth estimators. 
Not using dual pixel views hinders the network's ability to find clear foreground-background separations resulting in smudged egdes~\cref{fig:qualitative}.

\textbf{Dual-Pixel based Disparity Estimation Baselines.}
We benchmark \textit{dp}MV with similar input (RGB+\textit{dp}) methods: DDDNet and DPDD
% Write briefly about each baseline & how our method compares
The rationale for choosing these MDE baselines with high representation power and massive training datasets is to demonstrate competitive or better disparity estimation fidelity while being \textit{practical} for deployment and downstream edge applications. 
Whereas, the main purpose for the \textit{dp}-baselines is to benchmark our \textit{dp}MV dataset and also provide a holistic comparison of the conventional disparity from dual pixel task.

\subsubsection{Evaluation Criteria}
\label{sec:affine_inv_metrics}       
We use affine invariant MAE ($AI(1)$) and affine invariant RMSE ($AI(2)$) for evaluation, similar to~\cite{punnappurath2020modeling}.
We also consider the number of parameters and the inference time to be significant factors for real-world use cases of such neural networks or kernel optimization-based methods.

\subsubsection{Quantitative Comparison and dpMV Benchmark}
All metrics are computed on a set of 145 images shown in~\cref{fig:all_dataset_IP_1},~\cref{fig:all_dataset_IP_2} and~\cref{fig:all_dataset_IP_3}.
The $CPU$ and $GPU$ runs are averaged on the same set, thrice for the GPU times and once for the CPU times.
Note that the times mentioned are per-image.
See~\cref{tab:benchmark_dpmv} for the quantitative benchmark on disparity estimation.

% \subsubsection{More Qualitative Results}
% See~\cref{fig:dp_disp_more}

\subsubsection{Ablation: Efficiency vs Accuracy}
In~\cref{tab:my_label_abl} we demonstrate the parameter and inference speed gains versus the drop in accuracy of our models. 

\subsubsection{Limitation. The Droplet Artifact due to Batch Normalization}
\label{sec:supp_batch_normalization}
Batch Normalization has been attributed to the water-droplet smudge artifact as first observed in styleGAN2~\cite{stylegan2} by Karras~\etal~\cite{stylegan3} (StyleGAN3).
Similarly, super-resolution methods like ESRGAN~\cite{esrgan} do not use batch normalization for any of the deep residual-in-residual blocks to maintain sharpness. 
\begin{figure}[h]
    \centering
    \includegraphics[width=0.99\columnwidth]{supp_imgs/dark_dp_est/limitation_styleGAN3.png}
    \caption{\textbf{Dark dp-disparity-networks' Limitation.} The water-droplet-like smudging that occurs for some estimations is attributed to the batch normalization layers in the decoder.}
    \label{fig:dark_dp_limitation}
\end{figure}
Similarly, we attribute this smudged or water-droplet effect in our dark-tiny-dp-disparity networks due to batch normalization layers in the decoder.
