# Supplementary material for: Stereo-Knowledge Distillation from dpMV to Dual Pixels for Light Field Video Reconstruction
Source: arXiv:2405.11823 source file (2024-05-20)
Supplement: Supplementary file 4 [file dataset.tex]

\section{\textit{dp}MV Dataset} 
\label{sec:dataset}
\begin{figure}[h]
    \centering
    \includegraphics[width=0.99\columnwidth]{supp_imgs/dataset/dataset_rig.png}
    \caption{\textbf{Dataset Capturing Rig:} Front and Back.}
    \label{fig:front_back_rig}
\end{figure}
\begin{figure}[h]
    \centering
    \includegraphics[width=0.9\columnwidth]{supp_imgs/dataset/fpsvsthreads.jpg}
    \caption{Maximum Capture $fps$ versus number of threads}
    \label{fig:capture_fps_number_of_threads}
\end{figure}

In this section, we highlight the categorized and annotated scenes and follow up by providing more details of the capturing, synchronization and storing procedure.

\subsection{Hardest Scene of dpMV}
\label{subsec:hardest_scene}
This scene contains extremely non-Lambertian surfaces, and reflective \& transmissive glass panels simultaneously.

\begin{figure}[ht]
    \centering
    \includegraphics[width=0.9\columnwidth]{supp_imgs/dataset/hardest_scene.png}
    \caption{\textbf{Hardest Transmissive, Reflective and Non-Lambertian Scene in \textit{dp}MV.} Even the dark stereo geometry teacher's disparity estimate ($d_{st}$) is \textit{poor} quality and untrue to the scene. 
    We never use this scene for training or testing purposes.
    }
    \label{fig:hardest_scene}
\end{figure}
\subsection{Transmissive, Reflective and Non-Lambertian Scenes}
Our methods are not designed for these scenes but we hope that the reflective-transmissive surface reconstruction community finds these scenes useful.

\subsection{Scene Categories} 
\textbf{One representative image for each scene (video) with the classification category is shown in~\cref{fig:all_dataset_IP_1},~\cref{fig:all_dataset_IP_2} and~\cref{fig:all_dataset_IP_3}.}
We consider the category as the 1-or-2-word caption of the entire video.

\subsection{Capturing Rig}
We show the front and back of our rig in~\cref{fig:front_back_rig}.

\subsection{Synchronization}
To synchronize capture across three devices, Simple Network Time Protocol (SNTP) is utilized. Phones obtain offsets from a public NTP server. A designated device acts as the master, determining the start time for capture across all devices. The master's chosen timestamp is sent to a web server, and other devices fetch this adjusted target timestamp to initiate capture simultaneously. To validate synchronization, we record a timer before capture and manually adjust frames post-capture if synchronization issues arise.

\subsection{Capture Frame Rate}
To optimize our capture process, an optimal frame rate is crucial. If the frame rate is too high, frame synchronization becomes challenging. The total time per frame involves both I/O time for storing the frame and processing time, including dual pixel quantization to 8 bits and JPEG compression~\cite{GargDualPixelsICCV2019_DPNet}. Processing multiple frames in parallel reduces processing time, thus increasing the supported frame rate. Empirically, using around 6 worker threads achieves the best performance, consistently reaching approximately 18 FPS without frame drops. However, performance decreases at higher CPU temperatures. Given that much of our dataset is captured outdoors with elevated temperatures, we capped the actual capture frame rate at 13 $fps$ (see~\cref{fig:capture_fps_number_of_threads}).

\subsection{Processing \textit{dp}-Frames}
The Pixel-4 phones provide dual pixel data at 10-bit resolution which are re-quantized to 8 bits and stored with JPEG compression. We minimize quantization loss similar to \cite{GargDualPixelsICCV2019_DPNet} by first re-scaling the data to $0-2^{16}$ and then compressing to 8-bit integer depth followed by quantization.

\begin{figure*}[ht]
    \centering
    \begin{subfigure}{0.9\textwidth}
        \includegraphics[width=\textwidth]{supp_imgs/dataset/nl_scenes_1.png}
    \end{subfigure}
    \hfill
    \begin{subfigure}{0.9\textwidth}
        \centering
        \includegraphics[width=0.7\textwidth]{supp_imgs/dataset/nl_scenes_2.png}
    \end{subfigure}
    \caption{\textbf{Transmissive, Reflective and Non-Lambertian Scenes of \textit{dp}MV.} The top row shows harder scenes compared to the bottom two. The last row predominantly focuses on visible light sources.}
    \label{fig:transmissive_reflective}
\end{figure*}
