# Supplementary material for: Stereo-Knowledge Distillation from dpMV to Dual Pixels for Light Field Video Reconstruction
Source: arXiv:2405.11823 source file (2024-05-20)
Supplement: Supplementary file 5 [file discuss.tex]

\section{Discussion}
\label{sec:discussion}
Through this supplementary, we have extended the motivation of our work and validated our direction \textit{with theory} to reach a hypothesis beneficial for dual-pixel solutions.
The hypothesis is elaborated upon and finally validated as we report the \textit{dp}MV benchmark, qualitative results, ablations, and comparisons on the dual-pixel disparity estimation comprehensively. We also provide our methodology, implementation details, and schematics for the same.
To further test the effectiveness of our dark knowledge hypothesis, we demonstrate a single-view light field video reconstruction method. 
In the process, we push the light field research forward by using dual pixels, showing the use of vision transformers for the first time and achieving the fastest and most temporally consistent light field videos. 
We provide the theory for simulating our dual pixel channels and homographic transforms. 
We show additional results, and experiments, discuss the appropriateness of softmax splatting for explicit disocclusion handling, and end the section with a demonstration of our method.
Finally, we show our dataset in detail with the categorized and captioned form in which it exists and will be released.

\begin{figure*}[htb!]
    \centering
    \begin{subfigure}{0.9\textwidth}
        \includegraphics[width=\textwidth]{supp_imgs/dataset/samples_1.png}
    \end{subfigure}
    \hfill
    \begin{subfigure}{0.9\textwidth}
        \includegraphics[width=\textwidth]{supp_imgs/dataset/samples_2.png}
    \end{subfigure}
    \caption{\textbf{\textit{dp}MV scenes - 1/3.} Except the hardest one shown in~\cref{subsec:hardest_scene}.}
    \label{fig:all_dataset_IP_1}
\end{figure*}

\begin{figure*}[hbt!]
    \centering
    \begin{subfigure}{0.9\textwidth}
        \includegraphics[width=\textwidth]{supp_imgs/dataset/samples_4.png}
    \end{subfigure}
    \hfill
    \begin{subfigure}{0.9\textwidth}
        \includegraphics[width=\textwidth]{supp_imgs/dataset/samples_5.png}
    \end{subfigure}
    \caption{\textbf{\textit{dp}MV scenes - 2/3.} Except the hardest one shown in~\cref{subsec:hardest_scene}.}
    \label{fig:all_dataset_IP_2}
\end{figure*}

\begin{figure*}[hbt!]
    \centering
    \begin{subfigure}{0.9\textwidth}
        \includegraphics[width=\textwidth]{supp_imgs/dataset/samples_3.png}
    \end{subfigure}
    \hfill
    \begin{subfigure}{0.9\textwidth}
        \includegraphics[width=\textwidth]{supp_imgs/dataset/samples_6.png}
    \end{subfigure}
    \caption{\textbf{\textit{dp}MV scenes - 3/3.} Except the hardest one shown in~\cref{subsec:hardest_scene}.}
    \label{fig:all_dataset_IP_3}
\end{figure*}

\clearpage
