# Supplementary material for: Stereo-Knowledge Distillation from dpMV to Dual Pixels for Light Field Video Reconstruction
Source: arXiv:2405.11823 source file (2024-05-20)
Supplement: Supplementary file 6 [file dual_pixels.tex]

\section{Motivation. Dual Pixels: A Boon and a Bane }
\label{sec:dp_explained_dof}

\textbf{Disparity Formulation in Dual Pixels.}
The disparity for a stereo pair with baseline $B$ at pixel $(x,y)$ in the left camera is given by $d^{st}_{x,y} = Bf/z$, where z is the depth at the pixel and $f$ is the focal length.
However, due to the introduction of the micro-lenslet array over the pixel sensor board and under the main lens, in addition to the tiny baseline of dual pixels, the equation for the disparity, similarly defined by Kim~\etal~\cite{spatio_bifocal} using the circle-of-confusion size ($b$), is given by: 
\begin{equation}
    d^{dp}_{x,y} = \alpha b = \alpha \frac{Af}{1 - f/z_f} (\frac{1}{z_f} - \frac{1}{z}) = p + \frac{q}{z}
    \label{eq:dp_disparity_equation}
\end{equation}
where, $A$ is the size of the main lens aperture, $z_f$ is the depth of the focus plane, $\alpha$ is a positive scale factor (\cref{fig:dp_dof_explainer}).
Note that this equation is affinely related to depth contrary to the stereo setup where they are directly inversely proportional.
We also solve for affine parameters for each dual-pixel disparity baseline and the inverse relation for monocular depth estimation to get affine-invariant metrics for disparity estimation in~\cref{tab:benchmark_dpmv}.

Nevertheless, when a camera operates in ultra-large depth-of-field or all-in-focus settings ($b \rightarrow 0$), dual pixel disparity is negligible ($d^{dp}_{x,y} \rightarrow 0$). 
This limitation necessitates capturing with \textit{defocus blur} to get disparity information~\cite{spatio_bifocal, refocus_wadwa_18}. 
This is not the case with stereo-camera setups to estimate disparity.
So, this necessitates the exploration of a solution that can utilize the dual pixel hardware while reaching stereo-accuracy in \textit{all} camera operating conditions. 

\begin{figure}[t]
    \centering
    \includegraphics[width=\columnwidth]{supp_imgs/dual_pixels/dual_pixel_explainer.png}
    \caption{\textbf{Dual Pixels have disparity \textit{only} in out-of depth-of-field of the camera or defocus deblur regions.} Image Courtesy: Kim~\etal~\cite{spatio_bifocal}}
    \label{fig:dp_dof_explainer}
\end{figure}

\textbf{Machine Learning for the Best of Both.}
The drawback of dual pixels is the need to capture with defocus blur. 
However, this might not always be possible with proprietary camera ISPs that stabilize and aim for all-in-focus shots.
Stereo camera setups need perfect synchronization and the hardware needed for integration in a small-scale device like a smartphone is plentiful, making it impractical even if it is more accurate.
Machine learning delivers the best of both worlds by distilling knowledge from stereo networks to dp-networks.
This helps dp-networks to understand the depth-of-field of the camera and utilize appropriate channels (RGB for within depth-of-field and dp for out-of depth-of-field).
