# Supplementary material for: Stereo-Knowledge Distillation from dpMV to Dual Pixels for Light Field Video Reconstruction
Source: arXiv:2405.11823 source file (2024-05-20)
Supplement: Supplementary file 7 [file lfvr.tex]

\section{More Light Field Video Reconstruction}
\label{sec:lfvr_supplement}

\subsection{Properties in a Nutshell}
Here, we re-iterate the properties of our method concisely.

\textbf{Zero-shot Cross Dataset Transfer:}
Most existing literature requires fine-tuning on other datasets before evaluation, so we believe zero-shot cross-dataset transfer is an important generalization property for end-user applications.

\textbf{Zero-shot Inference of Higher (than training) Spatial-Angular Resolutions}
Our reconstructions remain geometrically consistent and our PSNR rises as the input spatial resolution increases. See figure 6 in main text and~\cref{tab:fig6_plot_values}.

\textbf{Implicit Disocclusion Handling}
We believe that if the feature extractor(s) understand the 3D scene well and have some context during training, they can learn to implicitly handle disocclusion by filling holes in extreme SAIs using the surroundings. 
Explicit hand-holding such as softmax-splatting~\cite{niklaus2020softmax} leads to a poorer 3D world understanding and often incorrectly splats foreground pixels to the background, see~\cref{sec:softmax_bad}.

\textbf{Fastest Inference and High Parameter Efficiency make our solution the most deployment fit to date.}
See the temporal consistency, parameters, and inference speed table in the main text.

\textbf{Highest Video LF Temporal Consistency.}
See \textit{supplementary slide 22} for video LF results.

\subsection{Full Model and Optimization Loop Figure}
The flow teacher $\flownet$ gets added after 100 training epochs with the geometry teacher. 
See~\cref{fig:full_arch} for a full model diagram alongside how the losses get distilled. The main text does not have the flow-teacher distillation loss schematic.

\begin{figure*}[ht]
    \centering
    \includegraphics[width=0.95\textwidth]{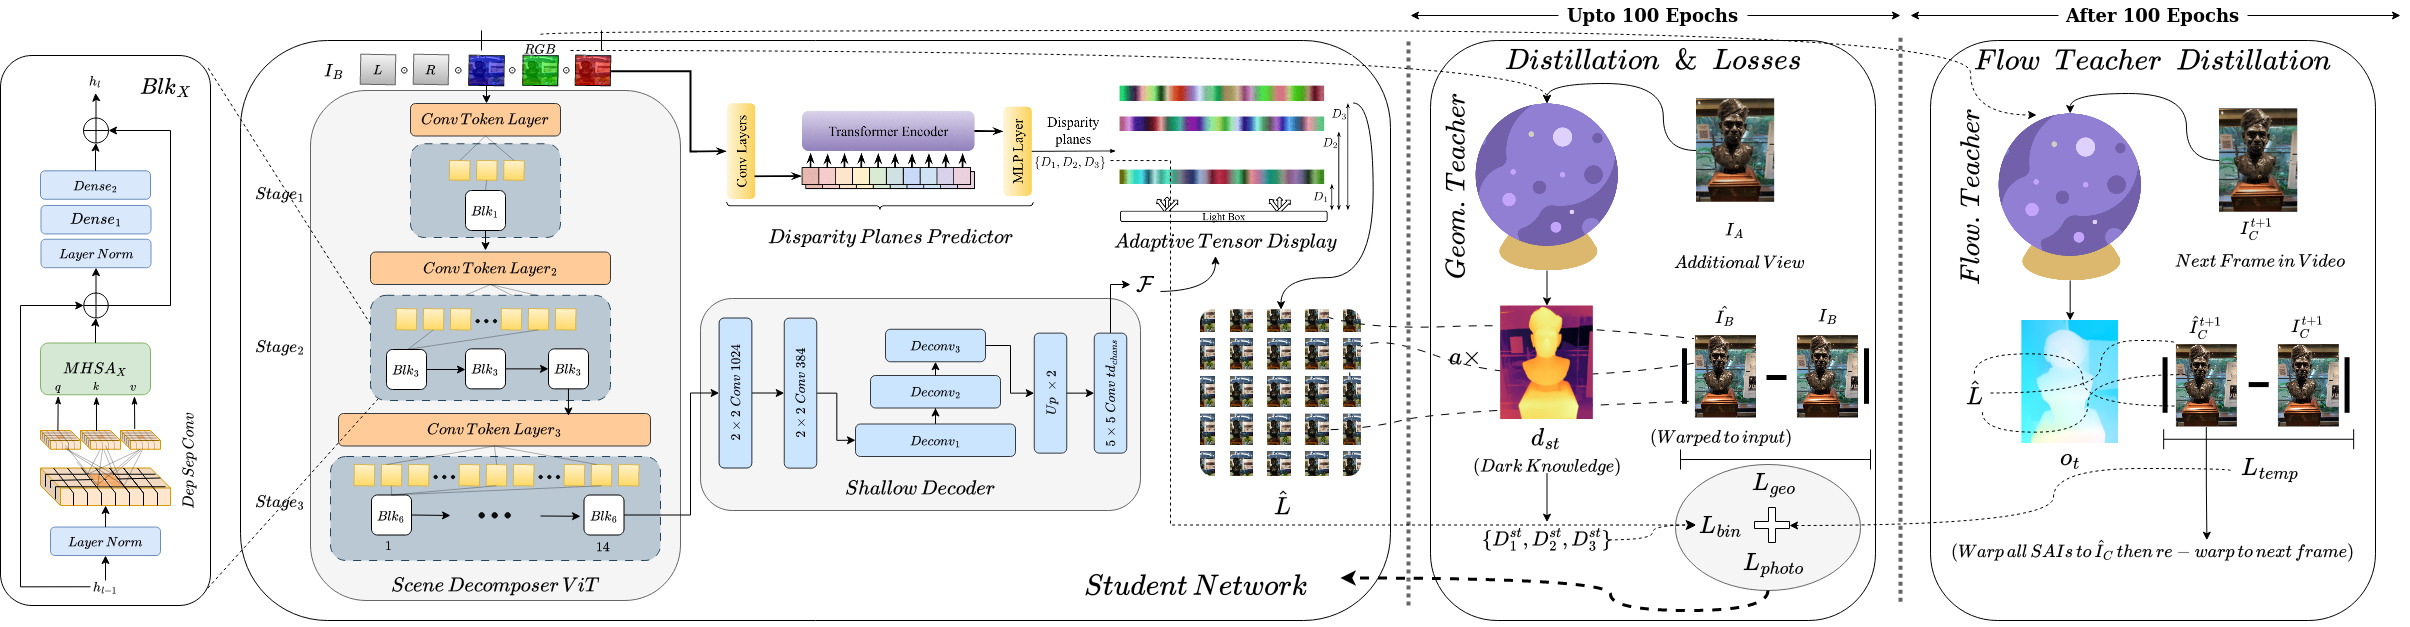}
    \caption{\textbf{Full Model Diagram with Losses.} Here, $\flownet$ takes the next video frame as input and computes an optical flow map $o_t$ using which all the warped-to-center SAIs ($\hat{I}_C$) are warped to the next video input frame, one by one.
The summation of the error gives the temporal loss.
Our method uses RAFT~\cite{raft_RAFT} as the flow-teacher ($\flownet$) and achieves the most temporally consistent video LFs.}
    \label{fig:full_arch}
\end{figure*}

\subsection{More Implementation Details}
% DeepSpeed's Zero-offloading-2~\cite{ren2021zerooffload} was initially explored but a simpler gradient accumulation of \textit{16-iterations} offered similar compute gains with a simpler training loop.
\textit{Extra losses tried.} D-SSIM~\cite{ssim} in conjunction with photometric loss. We discovered that it was not needed since the main scene decomposer could preserve global and local structure effectively so we chose to keep it simple. 
Additionally, we tried the softmax-splatting~\cite{niklaus2020softmax} formulation like Mono~\cite{eccv_22_monoLFVR} but only for boundary operating conditions of the dark knowledge scaling factor ($a > 3$).
The loss splatted foreground pixels to the background giving a sheared look to SAIs .

\subsection{Why explicit disocclusion handling or softmax-splatting~\cite{niklaus2020softmax} is inappropriate for LF reconstruction}
\label{sec:softmax_bad}
Softmax splatting~\cite{niklaus2020softmax} based disocclusion handling splats pixels, forcibly, from the foreground to the background. 
Notice how the ear stretches out as the baseline of generated LF increases in \textit{supplementary slide number 18} (Demonstration of the same phenomenon through GIFs).

\subsection{Simulating Dual Pixel Channels from Ground Truth Light Fields}
We average the adjacent SAI with the center view to get a dual-pixel channel. 
This works to an extent as the GT light fields do not have an adjacent SAI baseline $> 2$ pixels. 
Averaging naively brings the \textit{dp}-channel baseline to sub-pixel levels ($< 1$).
\begin{equation}
    dp_L = \frac{L(\mathbf{-1}) + L(\mathbf{0})}{2}
    \And
    dp_R = \frac{L(\mathbf{0}) + L(\mathbf{1})}{2}
\end{equation}
where $L(\mathbf{0})$ is the central view of the ground truth or captured Light Field(LF). $L(\mathbf{-1})$ and $L(\mathbf{1})$ correspond to the adjacent left and right sub-aperture views of the same LF.
See \textit{supplementary slide 20} for simulated dp-channels' GIF (sub-pixel baseline).

\subsection{Homography: To convert Image-LFs to Video-LFs for temporal consistency evaluation}
While we only require adjacent RGBs from a video sequence for the flow teacher that trains the LF student network to be temporally consistent; we require ground-truth $LF$ video to quantitatively evaluate the estimated $LF$ videos during the evaluation of temporal consistency.
For this, we generate $5$D $LF$ videos from a single $4$D $LF$ image.

Consider a $4$D $LF$ image of the form $L(x,y,u,v)$ where $(x,y)$ are the spatial co-ordinates and $(u,v)$ are the angular co-ordinates.
While simulating the video sequence, we assume a model of multiple pinhole cameras located at the co-ordinates $(u,v)$ from which individual views of the $LF$ are captured.
% Simulating a camera motion through the given light-field is equivalent to resampling the given $4$D light-field function and projecting it to the desired camera~\cite{lumentut2019fast,lfdeblurringlumentut}.
We consider the 6-DoF camera motion with translation and rotation defined as $P(t) = [\tx, \ty, \tz]$ and $R(t) = [\rx, \ry, \rz]$, respectively.
We consider the stereo camera located at the two views $(0,v_m)$ and $(U,v_m)$.
For the given 6-DoF translation and rotation $P(t)$ and $R(t)$ respectively, the left view at time $t$ is given by,
\begin{align}
    \leftframe &= L(x^j, y^j, p_x^i(t)-x^j\tz, v_m + p_y^i(t)-y^j\tz) \\
    x^j &= (x - U/2) \cos{\rz} - y \sin(\rz) + U/2 \\
    y^j &= (x - U/2) \sin{\rz} + y \cos(\rz) \\
    p_x^i&(t) = \tx + f\rx \\
    p_y^i&(t) = \ty + f\ry
\end{align}
where $f$ is the focal length of the camera.
Similarly, the right view of the camera is given by,
\begin{align}
    \rightframe = L(x^j, y^j, U + p_x^i(t)-x^j\tz, v_m + p_y^i(t)-y^j\tz)
    % x^j = (x - U/2) \cos{\rz} - y \sin(\rz) + U/2
    % y^j = (x - U/2) \sin{\rz} + y \cos(\rz) \\
    % p_x^i(t) = \tx + f\rx \\
    % p_x^i(t) = \ty + f\ry
\end{align}

% \subsection{Varying angular \& spatial resolution outputs}

\subsection{Quantitative Evaluation of Zero-Shotting Higher Spatial Resolutions than training}
In~\cref{tab:fig6_plot_values}, we report the exact values of the plot shown in Fig 6 (main text) that demonstrates how our method synthesizes geometrically consistent LFs even at very high, unseen, and modern-day required resolutions like close to Standard Definition ($480 \times 640$).

\begin{table}[ht]
    \centering
    \caption{\textbf{Zero-Shotting Higher Spatial Resolutions} - Quantitative Results (Fig 6 plot in main text)}
    \begin{tabular}{lcccccc}
        \toprule
        
        \textbf{Res.} & \cite{Niklaus_Ken_Burns} &  \textbf{Li} & \textbf{Li+}\cite{Ranftl2020} & \textbf{Mono} & \textbf{Mono-R} & \textbf{Ours}  \\
        
        \midrule
        $192^2$ & 20.564 & 26.285 & 25.730 & 26.369 & \textbf{26.622} & 25.754  \\  
        
        $256^2$ & 20.386 & 26.232 & 26.123 & 26.773 & \textbf{27.053} & 26.481 \\  
        
        $384^2$ & 16.574 & 26.056 & 26.033 &  26.748 & 27.023 & \textbf{27.082 } \\  
        
        $480^2$ & 16.444 & 25.928 & 25.926 & 26.791 & 27.249  & \textbf{27.304}  \\  
        % \midrule
        \bottomrule
    \end{tabular}
    \label{tab:fig6_plot_values}
\end{table}

\begin{figure}[ht]
    \centering
    \includegraphics[width=0.99\columnwidth]{supp_imgs/lfvr/epi_SD_1.5x.png}
    \caption{\textbf{Geometrically Consistent EPIs at Higher (Zero Shot) Spatial Resolutions} with the LF baseline, dark knowledge scaling hyperparameter ($a = 1.5$) larger than GT LF baselines.}
    \label{fig:ZS_higher_res}
\end{figure}

\begin{figure}[ht]
    \centering
    \includegraphics[width=0.6\columnwidth]{supp_imgs/lfvr/extreme_a_4.png}
    \caption{\textbf{Limitaion. Extremely Large Dark Knowledge Scaling Factor.} $a = 4$ produces artifacts around foreground-background separation regions in extreme sub-aperture images (SAIs) }
    \label{fig:limitation_1}
\end{figure}

\subsection{Qualitative Evaluation of Zero-Shotting Higher Spatial Resolutions - Geometrically Consistent EPIs}
Our method achieves geometric, Consistent epipolar images (EPIs) at Standard Definition ($480 \times 640$).
% \begin{figure*}[ht]
%     \centering
%     \includegraphics[width=0.99\textwidth]{supp_imgs/lfvr/xr_app1.png}
%     \caption{\textbf{XR Applications} of Our Reconstructed Light Fields.}
%     \label{fig:xr_applications}
% \end{figure*}

\subsection{More Applications - Refocusing \& Novel View Synthesis}
Refocusing is shown in~\cref{fig:refocus}.
Novel view synthesis crops are shown in~\cref{fig:nvs_all}.

\begin{figure}[ht]
    \centering
    \begin{subfigure}{0.46\textwidth}
        \includegraphics[width=\textwidth]{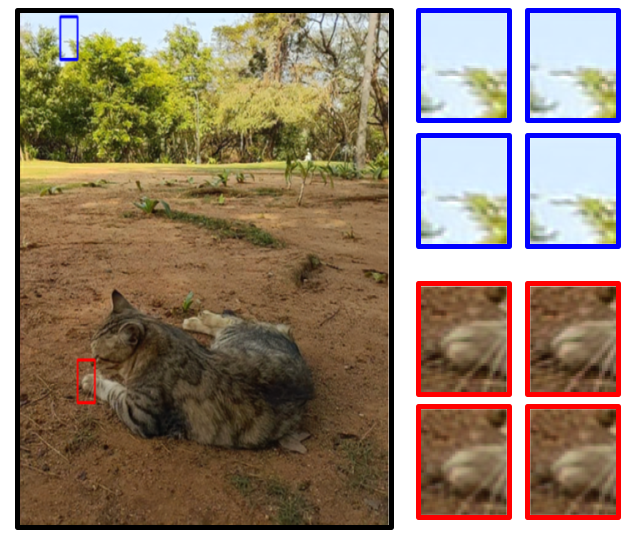}
    \end{subfigure}
    \hfill
    \centering
    \begin{subfigure}{0.46\textwidth}
        \includegraphics[width=\textwidth]{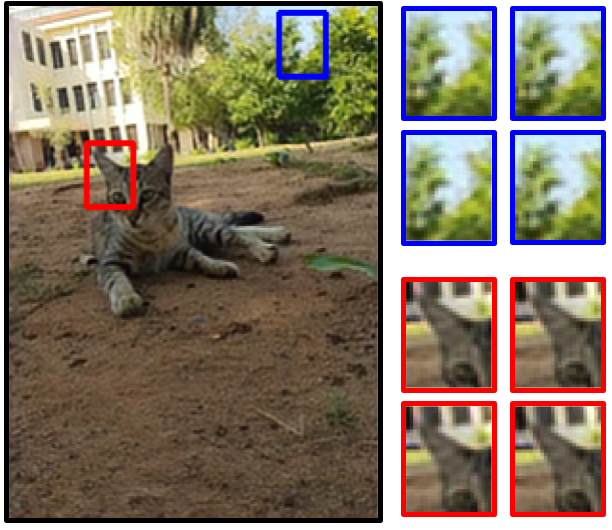}
    \end{subfigure}
    \caption{\textbf{Novel View Synthesis} using reconstructed Light Fields. The shift in crops exists as they are extreme Top-Left, top-right, bottom-left, and bottom-right SAIs of the LF respectively.}
    \label{fig:nvs_all}
\end{figure}

\subsection{Limitation 1 - Extreme Dark Knowledge Scaling} 
The failure mode occurs due to stretching our dark knowledge disparity estimate ($d_{st}$) too much.
This phenomenon is observed for values of $a > 3$.
Extreme SAIs suffer due to ineffective dual pixel guidance as the uneven stretching of dark knowledge becomes more prominent, see~\cref{fig:limitation_1}

\subsection{Limitation 2 - Extremely Transmissive and Reflective Surfaces}
Our method is not designed to reconstruct transmissive and extremely reflective surfaces.
\textit{dp}MV has a few such scenes shown in~\cref{fig:transmissive_reflective} and~\cref{fig:hardest_scene}.
Flickering artifacts can also be seen in reconstructed LFs for extremely shiny or non-Lambertian scenes.

% \subsection{Extreme Values of Dark Knowledge Scaling Hyper-parameter}
