# Supplementary material for: Stereo-Knowledge Distillation from dpMV to Dual Pixels for Light Field Video Reconstruction
Source: arXiv:2405.11823 source file (2024-05-20)
Supplement: Supplementary file 8 [file related.tex]

\section{Extended Related Work}
\label{sec:extended_related}
\subsection{Disparity Estimation}
We surveyed three input-type methods for disparity estimation: monocular, dual-pixel, and stereo input.
The stereo-input methods were surveyed to select optimal dark-teachers for our distillation hypothesis while the others serve the purpose of baselines or noteworthy ideas.
We omit multi-view stereo methods like COLMAP~\cite{colmap_COLMAP}.

\textit{Monocular Depth Estimation Methods.}
Since disparity and depth are inversely proportional and can be estimated to a relatively accurate degree, we use and find in literature, mostly depth-based networks including the likes of Dense Prediction Transformer by Ranftl~\etal~\cite{Ranftl2020}, MiDaS~\cite{midas}, AdaBins~\cite{AdaBinsBhat} and ZoeDepth~\cite{zoeDepth}, both by Bhat~\etal.
The recent massively yet weakly supervised method Depth-Anything~\cite{depth_anything} method is by far the highest fidelity. 
We use it as a baseline for comparison.

\textit{Dual Pixel Methods.}
With the ubiquity of dual-pixel sensor smartphones, originally for auto-focusing, interest has risen in extracting disparity arising from the defocus blur.
DDDNet~\cite{Pan_2021_CVPR_DDDNet_DP_Disp}, DPNet~\cite{GargDualPixelsICCV2019_DPNet}, and DPDNet~\cite{abuolaim2020defocus_michaelBrownECCV} explored neural-network-based approaches.
While, Xin~\etal~\cite{Xin_2021_ICCV_dual_pixel_cmu}, DPDD~\cite{punnappurath2020modeling}, Wadhwa~\etal~\cite{refocus_wadwa_18} and Kim~\etal~\cite{spatio_bifocal} are purely optimization-based approaches thus requiring no-training data or a neural network.
Kim~\etal recently outperformed most optimization-based methods.
We contribute 4 mobile performant dp-disparity estimation neural network solutions using our dark knowledge distillation hypothesis.

\textit{Stereo Methods}
Disparity estimation or stereo matching has been a long-standing problem in computer vision and relies on effective feature matching and triangulation. 
Many deep learning-based methods have emerged that rely on warping, feature matching, cost-volume regression etc. 
Some methods include: ACVNet~\cite{xu2022attention_ACVNet}, Graft-PSM~\cite{graft_psm_net}, IGEV~\cite{xu2023iterative_igev}, CFNet~\cite{CF_Net_disp}, PSMNet~\cite{psmNet}, GA-Net~\cite{GA_Net}, AANet~\cite{AANet}, RAFT-Stereo~\cite{raft_stereo} and CREStereo~\cite{creStereo}.
Even transformer-based methods like STTR~\cite{STTR} and Unimatch or GMStereo~\cite{xu2023unifying_unimatch} exist. 
Unimatch won the Argoverse Challenge (CVPR-Workshop 2022 Autonomous Driving Challenge) even though it was pretrained on a synthetic dataset~\cite{sceneflow_dataset} thus showing remarkable real-world domain adaptation. 
This transformer-based network was fitting and unconstrained, thus making it a \textit{highly suitable} candidate for our \textit{dark knowledge geometry teacher} in the light field reconstruction task.

\begin{figure*}[ht]
    \centering
    \includegraphics[width=0.9\textwidth]{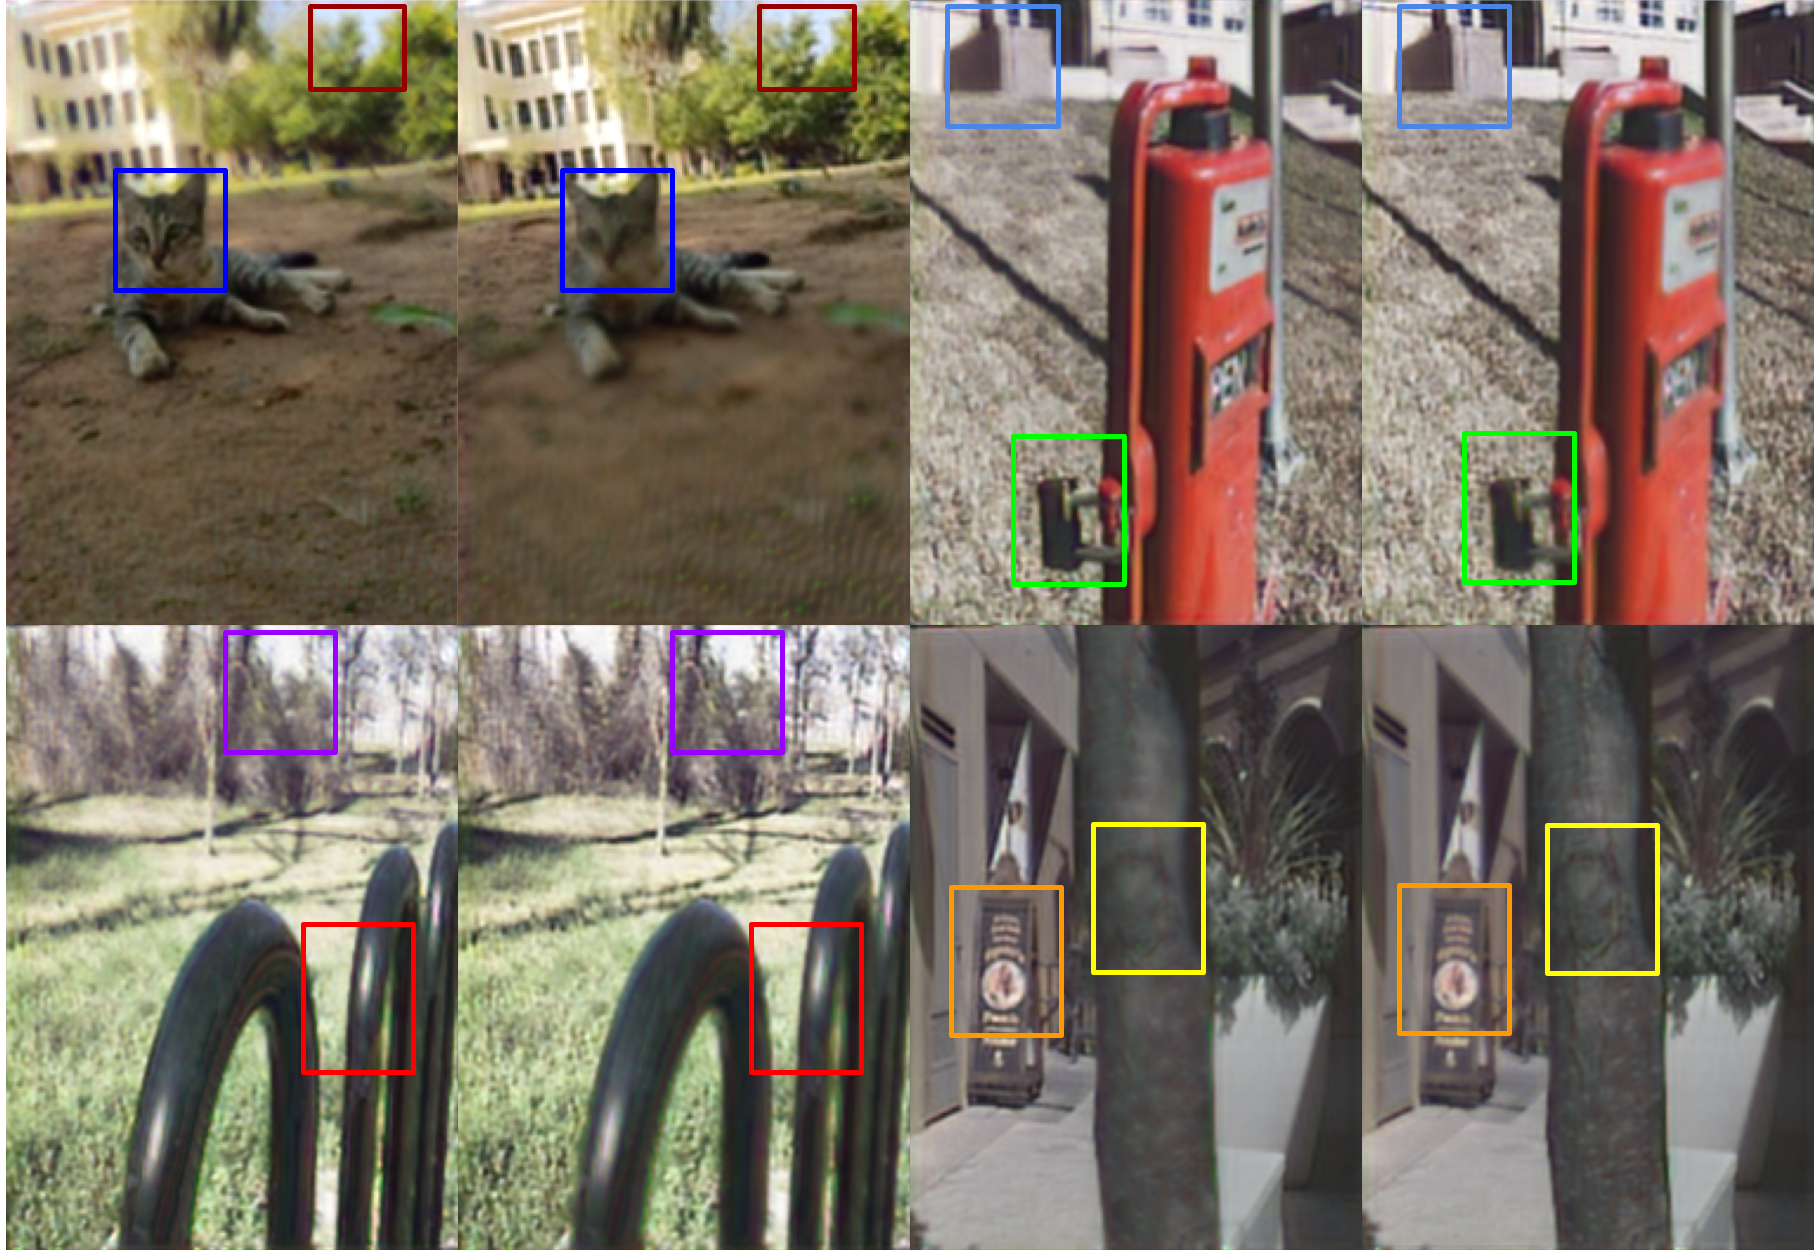}
    \caption{\textbf{Refocusing of our reconstructed light fields}. Note that the cat scene is from dpMV with real dual pixels while the others are from simulated dp-channels (GT LFdatasets)}
    \label{fig:refocus}
\end{figure*}

\subsection{Radiance Fields versus Light Fields}
\label{subsec:lf_vs_rf}
Even though Mildenhall \etal introduced the Local Light Field Fusion method \cite{LocalLF_fusion_2020} which eventually led them to an alternate, higher-fidelity seminal approach for novel view synthesis using radiance fields, colloquially known as NeRFs~\cite{mildenhall2020nerf, du2021nerflow, Dynamic_NeRF_Facial_Avatar, space_time_NeRF, dNeRF}, these approaches require integration along the rays to compute the intensity and opacity of a point in 3D space leading to a significant inference-time overhead. 
Additionally, a large set of overlapping inputs (upwards of 25) and cumbersome manual pre-processing using COLMAP for camera-pose estimation plagues them too. 
This is not practical for real scenarios where the user has a single shot at capturing a scene, for example, a flying bird.
Although, methods like pixelNeRF \cite{yu2021pixelnerf} and SinNeRF \cite{Xu_2022_SinNeRF} are singular view-based RF methods, they either work on simplistic objects or have prohibitive pre-training and inference times of up to 12 hours per scene. 
This significant time translates to all other downstream post-processing applications for every scene as NeRFs overfit/optimize MLPs to a scene. 
This makes RF-based methods totally infeasible for on-device applications whereas LF-based methods infer unseen scenes within mili-seconds. 
There have been significant efforts to eliminate this time drawback of RF methods and most speed-ups reduce the sampling points along a ray, but the issue of iterative sampling during ray-marching still persists. 
Recognizing this drawback, Wang \etal \cite{rf_2_lf} distilled an implicit 3D representation from a conventional NeRF model to a Neural LF model. 
Wang \etal observed a 30$\times$ speed-up with higher fidelity reconstructions but still needed intensive computations. 
InstantNGP~\cite{mueller2022instant_ngp},  MipNeRFs \cite{barron2021mipnerf} and the recent seminal 3D Gaussian Splatting method by Kerbl \etal \cite{kerbl3Dgaussians} present high-fidelity $120$+ fps renderings but still require an initial camera-pose estimation or 3D point cloud initialization. 
Per-scene optimization times of at least 20 minutes on sophisticated high-end graphics hardware are simply not possible for current smartphones, thus reiterating the practicality of learning explicit light fields as significantly faster and qualitatively better alternatives for non-deforming scenes~\cite{yu2023dylin}. 
To that end, we present the fastest Light Field Reconstruction method.

\subsection{Resurgence of Light Field Displays}
Light Fields have garnered interest mostly due to the availability of 3D-viewing hardware or 3D displays like Fovi3D, LumiPad and AR glasses from CREAL which are purely based on LF technology and enable interactive control (XR) as well.
