# Supplementary material for: Stereo-Knowledge Distillation from dpMV to Dual Pixels for Light Field Video Reconstruction
Source: arXiv:2405.11823 source file (2024-05-20)
Supplement: Supplementary file 9 [file repos.tex]

\section{Reproducibility}
\label{sec:reproducability}
The codebase for this paper is organized into three separate repositories (anonymous for now): 
Light Field Video Reconstruction, Dark tiny-dp-disparity networks and the Tuned-geometry-teacher in \href{https://github.com/ANonyMouxe/dp-LFVR}{dp-LFVR}, \href{https://github.com/ANonyMouxe/dark-dp-nets}{dark-dp-nets} and \href{https://github.com/ANonyMouxe/Dark-Knowledge-Tuned-Geometry-Teacher}{Dark-Knowledge-Tuned-Geometry-Teacher}.

\textbf{LFVR Implementation detail correction and addendum.} The light field reconstruction method uses a \textit{simulated} batch size of 16 using gradient accumulation instead of an actual batch size of 1. 
\textit{Addendum.} A fully PyTorch-Lightning codebase with DeepSpeed Zero-Offloading~\cite{ren2021zerooffload} for horizontal and extremely efficient sharding is under development and will be released upon publication.
